# Supplementary material for: Common Pairs of Graphs
Source: arXiv:2208.02045 ancillary file (2023-06-24)
Supplement: Supplementary file 1 [file commonExtraAppendices.pdf]

# Common Pairs of Graphs: Appendices

Natalie Behague, Natasha Morrison and Jonathan A. Noel

June 23, 2023

## A Verification of Flag Algebra Proof of Theorem 1.11 for $(p_1, p_2) = (1/2, 1/2)$

We verify the inequality in Lemma 5.8 with $(p_1, p_2) = (1/2, 1/2)$ and $(H_1, H_2) = (C_4, C_5)$ for each graph $J$ on 5 vertices. There are 34 such graphs, labelled $J_1$ to $J_{34}$.

$J_1$ : 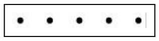

$$\begin{aligned}
&\frac{t_{\mathrm{inj}}(C_4, J_1)}{4(1/2)^3} + \frac{t_{\mathrm{inj}}(C_5, \overline{J_1})}{5(1/2)^4} - \frac{120}{120} \cdot A_1(1,1) \\
&= \frac{0}{120 \cdot 4(1/2)^3} + \frac{120}{120 \cdot 5(1/2)^4} - \frac{120}{120} \cdot \frac{25704}{8640} \\
&= \frac{9}{40}.
\end{aligned}$$

$J_2$ : 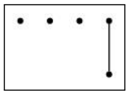

$$\begin{aligned}
&\frac{t_{\mathrm{inj}}(C_4, J_2)}{4(1/2)^3} + \frac{t_{\mathrm{inj}}(C_5, \overline{J_2})}{5(1/2)^4} - \frac{12}{120} \cdot A_1(1,1) - \frac{12}{120} \cdot A_1(1,2) - \frac{12}{120} \cdot A_1(1,3) - \frac{12}{120} \cdot A_1(1,4) \\
&\quad - \frac{12}{120} \cdot A_1(2,1) - \frac{12}{120} \cdot A_1(3,1) - \frac{12}{120} \cdot A_1(4,1) - \frac{12}{120} \cdot A_2(1,1) \\
&= \frac{0}{120 \cdot 4(1/2)^3} + \frac{60}{120 \cdot 5(1/2)^4} - \frac{12}{120} \cdot \frac{25704}{8640} - \frac{12}{120} \cdot \frac{6806}{8640} - \frac{12}{120} \cdot \frac{6806}{8640} - \frac{12}{120} \cdot \frac{6806}{8640} \\
&\quad - \frac{12}{120} \cdot \frac{6806}{8640} - \frac{12}{120} \cdot \frac{6806}{8640} - \frac{12}{120} \cdot \frac{6806}{8640} - \frac{12}{120} \cdot \frac{52260}{8640} \\
&= \frac{9}{40}.
\end{aligned}$$

$J_3$ : 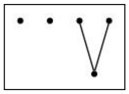

$$\frac{t_{\mathrm{inj}}(C_4, J_3)}{4(1/2)^3} + \frac{t_{\mathrm{inj}}(C_5, \overline{J_3})}{5(1/2)^4} - \frac{4}{120} \cdot A_1(1,2) - \frac{4}{120} \cdot A_1(1,3) - \frac{4}{120} \cdot A_1(1,4) - \frac{4}{120} \cdot A_1(1,5)$$

$$- \frac{4}{120} \cdot A_1(1,6) - \frac{4}{120} \cdot A_1(1,7) - \frac{4}{120} \cdot A_1(2,1) - \frac{4}{120} \cdot A_1(2,2) - \frac{4}{120} \cdot A_1(3,1) - \frac{4}{120} \cdot A_1(3,3)$$
$$- \frac{4}{120} \cdot A_1(4,1) - \frac{4}{120} \cdot A_1(4,4) - \frac{4}{120} \cdot A_1(5,1) - \frac{4}{120} \cdot A_1(6,1) - \frac{4}{120} \cdot A_1(7,1) - \frac{4}{120} \cdot A_2(1,2)$$
$$- \frac{4}{120} \cdot A_2(1,3) - \frac{4}{120} \cdot A_2(2,1) - \frac{4}{120} \cdot A_2(3,1) - \frac{4}{120} \cdot A_3(1,1)$$
$$= \frac{0}{120 \cdot 4(1/2)^3} + \frac{20}{120 \cdot 5(1/2)^4} - \frac{4}{120} \cdot \frac{6806}{8640} - \frac{4}{120} \cdot \frac{6806}{8640} - \frac{4}{120} \cdot \frac{6806}{8640} + \frac{4}{120} \cdot \frac{8112}{8640}$$
$$+ \frac{4}{120} \cdot \frac{8112}{8640} + \frac{4}{120} \cdot \frac{8112}{8640} - \frac{4}{120} \cdot \frac{6806}{8640} - \frac{4}{120} \cdot \frac{10512}{8640} - \frac{4}{120} \cdot \frac{6806}{8640} - \frac{4}{120} \cdot \frac{10512}{8640}$$
$$- \frac{4}{120} \cdot \frac{6806}{8640} - \frac{4}{120} \cdot \frac{10512}{8640} + \frac{4}{120} \cdot \frac{8112}{8640} + \frac{4}{120} \cdot \frac{8112}{8640} + \frac{4}{120} \cdot \frac{8112}{8640} - \frac{4}{120} \cdot \frac{4029}{8640}$$
$$- \frac{4}{120} \cdot \frac{4029}{8640} - \frac{4}{120} \cdot \frac{4029}{8640} - \frac{4}{120} \cdot \frac{4029}{8640} - \frac{4}{120} \cdot \frac{40104}{8640}$$
$$= \frac{9}{40}.$$

$J_4$ : 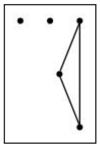

$$\frac{t_{\mathrm{inj}}(C_4, J_4)}{4(1/2)^3} + \frac{t_{\mathrm{inj}}(C_5, \overline{J_4})}{5(1/2)^4} - \frac{12}{120} \cdot A_1(2,2) - \frac{12}{120} \cdot A_1(3,3) - \frac{12}{120} \cdot A_1(4,4) - \frac{12}{120} \cdot A_2(1,5)$$

$$- \frac{12}{120} \cdot A_2(5,1) - \frac{12}{120} \cdot A_4(1,1)$$
$$= \frac{0}{120 \cdot 4(1/2)^3} + \frac{0}{120 \cdot 5(1/2)^4} - \frac{12}{120} \cdot \frac{10512}{8640} - \frac{12}{120} \cdot \frac{10512}{8640} - \frac{12}{120} \cdot \frac{10512}{8640} + \frac{12}{120} \cdot \frac{33264}{8640}$$
$$+ \frac{12}{120} \cdot \frac{33264}{8640} - \frac{12}{120} \cdot \frac{15552}{8640}$$
$$= \frac{9}{40}.$$

$J_5$ : 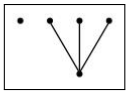

$$\frac{t_{\text{inj}}(C_4,J_5)}{4(1/2)^3}+\frac{t_{\text{inj}}(C_5,\overline{J_5})}{5(1/2)^4}-\frac{6}{120}\cdot A_1(1,5)-\frac{6}{120}\cdot A_1(1,6)-\frac{6}{120}\cdot A_1(1,7)-\frac{6}{120}\cdot A_1(1,8)$$

$$-\frac{6}{120}\cdot A_1(5,1)-\frac{6}{120}\cdot A_1(6,1)-\frac{6}{120}\cdot A_1(7,1)-\frac{6}{120}\cdot A_1(8,1)-\frac{6}{120}\cdot A_2(2,2)-\frac{6}{120}\cdot A_2(3,3)$$

$$-\frac{6}{120}\cdot A_3(1,2)-\frac{6}{120}\cdot A_3(2,1)$$

$$=\frac{0}{120\cdot 4(1/2)^3}+\frac{0}{120\cdot 5(1/2)^4}+\frac{6}{120}\cdot\frac{8112}{8640}+\frac{6}{120}\cdot\frac{8112}{8640}+\frac{6}{120}\cdot\frac{8112}{8640}+\frac{6}{120}\cdot\frac{21786}{8640}$$

$$+\frac{6}{120}\cdot\frac{8112}{8640}+\frac{6}{120}\cdot\frac{8112}{8640}+\frac{6}{120}\cdot\frac{8112}{8640}+\frac{6}{120}\cdot\frac{21786}{8640}-\frac{6}{120}\cdot\frac{19224}{8640}-\frac{6}{120}\cdot\frac{19224}{8640}$$

$$-\frac{6}{120}\cdot\frac{7458}{8640}-\frac{6}{120}\cdot\frac{7458}{8640}$$

$$=\frac{9}{40}.$$

$J_6$ : 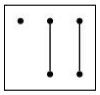

$$\frac{t_{\text{inj}}(C_4,J_6)}{4(1/2)^3}+\frac{t_{\text{inj}}(C_5,\overline{J_6})}{5(1/2)^4}-\frac{8}{120}\cdot A_1(2,3)-\frac{8}{120}\cdot A_1(2,4)-\frac{8}{120}\cdot A_1(3,2)-\frac{8}{120}\cdot A_1(3,4)$$

$$-\frac{8}{120}\cdot A_1(4,2)-\frac{8}{120}\cdot A_1(4,3)-\frac{8}{120}\cdot A_2(1,1)-\frac{8}{120}\cdot A_2(1,4)-\frac{8}{120}\cdot A_2(4,1)$$

$$=\frac{0}{120\cdot 4(1/2)^3}+\frac{40}{120\cdot 5(1/2)^4}+\frac{8}{120}\cdot\frac{1080}{8640}+\frac{8}{120}\cdot\frac{1080}{8640}+\frac{8}{120}\cdot\frac{1080}{8640}+\frac{8}{120}\cdot\frac{1080}{8640}$$

$$+\frac{8}{120}\cdot\frac{1080}{8640}+\frac{8}{120}\cdot\frac{1080}{8640}-\frac{8}{120}\cdot\frac{52260}{8640}-\frac{8}{120}\cdot\frac{31650}{8640}-\frac{8}{120}\cdot\frac{31650}{8640}$$

$$=\frac{9}{40}.$$

$J_7$ : 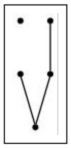

$$\frac{t_{\text{inj}}(C_4,J_7)}{4(1/2)^3}+\frac{t_{\text{inj}}(C_5,\overline{J_7})}{5(1/2)^4}-\frac{2}{120}\cdot A_1(2,3)-\frac{2}{120}\cdot A_1(2,4)-\frac{2}{120}\cdot A_1(2,5)-\frac{2}{120}\cdot A_1(2,6)$$

$$-\frac{2}{120}\cdot A_1(3,2)-\frac{2}{120}\cdot A_1(3,4)-\frac{2}{120}\cdot A_1(3,5)-\frac{2}{120}\cdot A_1(3,7)-\frac{2}{120}\cdot A_1(4,2)-\frac{2}{120}\cdot A_1(4,3)$$
$$-\frac{2}{120}\cdot A_1(4,6)-\frac{2}{120}\cdot A_1(4,7)-\frac{2}{120}\cdot A_1(5,2)-\frac{2}{120}\cdot A_1(5,3)-\frac{2}{120}\cdot A_1(6,2)-\frac{2}{120}\cdot A_1(6,4)$$
$$-\frac{2}{120}\cdot A_1(7,3)-\frac{2}{120}\cdot A_1(7,4)-\frac{2}{120}\cdot A_2(1,2)-\frac{2}{120}\cdot A_2(1,3)-\frac{2}{120}\cdot A_2(1,6)-\frac{2}{120}\cdot A_2(1,7)$$
$$-\frac{2}{120}\cdot A_2(2,1)-\frac{2}{120}\cdot A_2(2,3)-\frac{2}{120}\cdot A_2(3,1)-\frac{2}{120}\cdot A_2(3,2)-\frac{2}{120}\cdot A_2(6,1)-\frac{2}{120}\cdot A_2(7,1)$$
$$-\frac{2}{120}\cdot A_3(1,3)-\frac{2}{120}\cdot A_3(1,4)-\frac{2}{120}\cdot A_3(3,1)-\frac{2}{120}\cdot A_3(4,1)$$
$$=\frac{0}{120\cdot 4(1/2)^3}+\frac{10}{120\cdot 5(1/2)^4}+\frac{2}{120}\cdot\frac{1080}{8640}+\frac{2}{120}\cdot\frac{1080}{8640}-\frac{2}{120}\cdot\frac{481}{8640}-\frac{2}{120}\cdot\frac{481}{8640}$$
$$+\frac{2}{120}\cdot\frac{1080}{8640}+\frac{2}{120}\cdot\frac{1080}{8640}-\frac{2}{120}\cdot\frac{481}{8640}-\frac{2}{120}\cdot\frac{481}{8640}+\frac{2}{120}\cdot\frac{1080}{8640}+\frac{2}{120}\cdot\frac{1080}{8640}$$
$$-\frac{2}{120}\cdot\frac{481}{8640}-\frac{2}{120}\cdot\frac{481}{8640}-\frac{2}{120}\cdot\frac{481}{8640}-\frac{2}{120}\cdot\frac{481}{8640}-\frac{2}{120}\cdot\frac{481}{8640}-\frac{2}{120}\cdot\frac{481}{8640}$$
$$-\frac{2}{120}\cdot\frac{481}{8640}-\frac{2}{120}\cdot\frac{481}{8640}-\frac{2}{120}\cdot\frac{4029}{8640}-\frac{2}{120}\cdot\frac{4029}{8640}+\frac{2}{120}\cdot\frac{7632}{8640}+\frac{2}{120}\cdot\frac{7632}{8640}$$
$$-\frac{2}{120}\cdot\frac{4029}{8640}+\frac{2}{120}\cdot\frac{5400}{8640}-\frac{2}{120}\cdot\frac{4029}{8640}+\frac{2}{120}\cdot\frac{5400}{8640}+\frac{2}{120}\cdot\frac{7632}{8640}+\frac{2}{120}\cdot\frac{7632}{8640}$$
$$-\frac{2}{120}\cdot\frac{11880}{8640}-\frac{2}{120}\cdot\frac{11880}{8640}-\frac{2}{120}\cdot\frac{11880}{8640}-\frac{2}{120}\cdot\frac{11880}{8640}$$
$$=\frac{9}{40}.$$

$J_8$ : 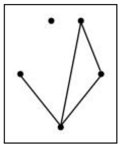

$$\frac{t_{\mathrm{inj}}(C_4,J_8)}{4(1/2)^3}+\frac{t_{\mathrm{inj}}(C_5,\overline{J_8})}{5(1/2)^4}-\frac{2}{120}\cdot A_1(2,5)-\frac{2}{120}\cdot A_1(2,6)-\frac{2}{120}\cdot A_1(3,5)-\frac{2}{120}\cdot A_1(3,7)$$
$$-\frac{2}{120}\cdot A_1(4,6)-\frac{2}{120}\cdot A_1(4,7)-\frac{2}{120}\cdot A_1(5,2)-\frac{2}{120}\cdot A_1(5,3)-\frac{2}{120}\cdot A_1(6,2)-\frac{2}{120}\cdot A_1(6,4)$$
$$-\frac{2}{120}\cdot A_1(7,3)-\frac{2}{120}\cdot A_1(7,4)-\frac{2}{120}\cdot A_2(1,5)-\frac{2}{120}\cdot A_2(1,8)-\frac{2}{120}\cdot A_2(2,2)-\frac{2}{120}\cdot A_2(2,5)$$
$$-\frac{2}{120}\cdot A_2(3,3)-\frac{2}{120}\cdot A_2(3,5)-\frac{2}{120}\cdot A_2(5,1)-\frac{2}{120}\cdot A_2(5,2)-\frac{2}{120}\cdot A_2(5,3)-\frac{2}{120}\cdot A_2(8,1)$$
$$-\frac{2}{120}\cdot A_3(1,5)-\frac{2}{120}\cdot A_3(1,6)-\frac{2}{120}\cdot A_3(5,1)-\frac{2}{120}\cdot A_3(6,1)-\frac{2}{120}\cdot A_4(1,2)-\frac{2}{120}\cdot A_4(1,3)$$

$$-\frac{2}{120}\cdot A_4(1,4)-\frac{2}{120}\cdot A_4(2,1)-\frac{2}{120}\cdot A_4(3,1)-\frac{2}{120}\cdot A_4(4,1)$$

$$=\frac{0}{120\cdot 4(1/2)^3}+\frac{0}{120\cdot 5(1/2)^4}-\frac{2}{120}\cdot\frac{481}{8640}-\frac{2}{120}\cdot\frac{481}{8640}-\frac{2}{120}\cdot\frac{481}{8640}-\frac{2}{120}\cdot\frac{481}{8640}$$
$$-\frac{2}{120}\cdot\frac{481}{8640}-\frac{2}{120}\cdot\frac{481}{8640}-\frac{2}{120}\cdot\frac{481}{8640}-\frac{2}{120}\cdot\frac{481}{8640}-\frac{2}{120}\cdot\frac{481}{8640}-\frac{2}{120}\cdot\frac{481}{8640}$$
$$-\frac{2}{120}\cdot\frac{481}{8640}-\frac{2}{120}\cdot\frac{481}{8640}+\frac{2}{120}\cdot\frac{33264}{8640}+\frac{2}{120}\cdot\frac{43440}{8640}-\frac{2}{120}\cdot\frac{19224}{8640}-\frac{2}{120}\cdot\frac{864}{8640}$$
$$-\frac{2}{120}\cdot\frac{19224}{8640}-\frac{2}{120}\cdot\frac{864}{8640}+\frac{2}{120}\cdot\frac{33264}{8640}-\frac{2}{120}\cdot\frac{864}{8640}-\frac{2}{120}\cdot\frac{864}{8640}+\frac{2}{120}\cdot\frac{43440}{8640}$$
$$+\frac{2}{120}\cdot\frac{10095}{8640}+\frac{2}{120}\cdot\frac{10095}{8640}+\frac{2}{120}\cdot\frac{10095}{8640}+\frac{2}{120}\cdot\frac{10095}{8640}-\frac{2}{120}\cdot\frac{4912}{8640}-\frac{2}{120}\cdot\frac{4912}{8640}$$
$$-\frac{2}{120}\cdot\frac{4912}{8640}-\frac{2}{120}\cdot\frac{4912}{8640}-\frac{2}{120}\cdot\frac{4912}{8640}-\frac{2}{120}\cdot\frac{4912}{8640}$$
$$=\frac{9}{40}.$$

$J_9$ : 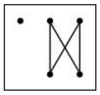

$$\frac{t_{\text{inj}}(C_4,J_9)}{4(1/2)^3}+\frac{t_{\text{inj}}(C_5,\overline{J_9})}{5(1/2)^4}-\frac{8}{120}\cdot A_1(5,5)-\frac{8}{120}\cdot A_1(6,6)-\frac{8}{120}\cdot A_1(7,7)-\frac{8}{120}\cdot A_2(2,3)$$
$$-\frac{8}{120}\cdot A_2(3,2)-\frac{8}{120}\cdot A_3(1,7)-\frac{8}{120}\cdot A_3(7,1)$$
$$=\frac{8}{120\cdot 4(1/2)^3}+\frac{0}{120\cdot 5(1/2)^4}-\frac{8}{120}\cdot\frac{11304}{8640}-\frac{8}{120}\cdot\frac{11304}{8640}-\frac{8}{120}\cdot\frac{11304}{8640}+\frac{8}{120}\cdot\frac{5400}{8640}$$
$$+\frac{8}{120}\cdot\frac{5400}{8640}+\frac{8}{120}\cdot\frac{17496}{8640}+\frac{8}{120}\cdot\frac{17496}{8640}$$
$$=\frac{9}{40}.$$

$J_{10}$ : 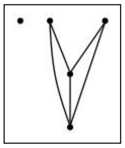

$$\frac{t_{\text{inj}}(C_4,J_{10})}{4(1/2)^3}+\frac{t_{\text{inj}}(C_5,\overline{J_{10}})}{5(1/2)^4}-\frac{4}{120}\cdot A_1(5,5)-\frac{4}{120}\cdot A_1(6,6)-\frac{4}{120}\cdot A_1(7,7)-\frac{4}{120}\cdot A_2(2,5)$$
$$-\frac{4}{120}\cdot A_2(3,5)-\frac{4}{120}\cdot A_2(5,2)-\frac{4}{120}\cdot A_2(5,3)-\frac{4}{120}\cdot A_2(5,5)-\frac{4}{120}\cdot A_3(1,8)-\frac{4}{120}\cdot A_3(8,1)$$

$$-\frac{4}{120}\cdot A_4(1,5)-\frac{4}{120}\cdot A_4(1,6)-\frac{4}{120}\cdot A_4(1,7)-\frac{4}{120}\cdot A_4(5,1)-\frac{4}{120}\cdot A_4(6,1)-\frac{4}{120}\cdot A_4(7,1)$$

$$\begin{aligned}=&\frac{8}{120\cdot 4(1/2)^3}+\frac{0}{120\cdot 5(1/2)^4}-\frac{4}{120}\cdot\frac{11304}{8640}-\frac{4}{120}\cdot\frac{11304}{8640}-\frac{4}{120}\cdot\frac{11304}{8640}-\frac{4}{120}\cdot\frac{864}{8640}\\&-\frac{4}{120}\cdot\frac{864}{8640}-\frac{4}{120}\cdot\frac{864}{8640}-\frac{4}{120}\cdot\frac{864}{8640}-\frac{4}{120}\cdot\frac{37140}{8640}+\frac{4}{120}\cdot\frac{33636}{8640}+\frac{4}{120}\cdot\frac{33636}{8640}\\&+\frac{4}{120}\cdot\frac{5166}{8640}+\frac{4}{120}\cdot\frac{5166}{8640}+\frac{4}{120}\cdot\frac{5166}{8640}+\frac{4}{120}\cdot\frac{5166}{8640}+\frac{4}{120}\cdot\frac{5166}{8640}+\frac{4}{120}\cdot\frac{5166}{8640}\end{aligned}$$

$$=\frac{9}{40}.$$

$J_{11}$ : 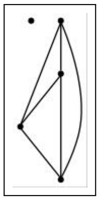

$$\begin{aligned}&\frac{t_{\mathrm{inj}}(C_4,J_{11})}{4(1/2)^3}+\frac{t_{\mathrm{inj}}(C_5,\overline{J_{11}})}{5(1/2)^4}-\frac{24}{120}\cdot A_2(5,5)-\frac{24}{120}\cdot A_4(1,8)-\frac{24}{120}\cdot A_4(8,1)\\&=\frac{24}{120\cdot 4(1/2)^3}+\frac{0}{120\cdot 5(1/2)^4}-\frac{24}{120}\cdot\frac{37140}{8640}+\frac{24}{120}\cdot\frac{14790}{8640}+\frac{24}{120}\cdot\frac{14790}{8640}\\&=\frac{9}{40}.\end{aligned}$$

$J_{12}$ : 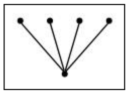

$$\begin{aligned}&\frac{t_{\mathrm{inj}}(C_4,J_{12})}{4(1/2)^3}+\frac{t_{\mathrm{inj}}(C_5,\overline{J_{12}})}{5(1/2)^4}-\frac{24}{120}\cdot A_1(1,8)-\frac{24}{120}\cdot A_1(8,1)-\frac{24}{120}\cdot A_3(2,2)\\&=\frac{0}{120\cdot 4(1/2)^3}+\frac{0}{120\cdot 5(1/2)^4}+\frac{24}{120}\cdot\frac{21786}{8640}+\frac{24}{120}\cdot\frac{21786}{8640}-\frac{24}{120}\cdot\frac{33852}{8640}\\&=\frac{9}{40}.\end{aligned}$$

$J_{13}$ : 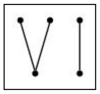

$$\frac{t_{\mathrm{inj}}(C_4,J_{13})}{4(1/2)^3}+\frac{t_{\mathrm{inj}}(C_5,\overline{J_{13}})}{5(1/2)^4}-\frac{4}{120}\cdot A_1(2,7)-\frac{4}{120}\cdot A_1(3,6)-\frac{4}{120}\cdot A_1(4,5)-\frac{4}{120}\cdot A_1(5,4)$$

$$-\frac{4}{120}\cdot A_1(6,3)-\frac{4}{120}\cdot A_1(7,2)-\frac{4}{120}\cdot A_2(1,4)-\frac{4}{120}\cdot A_2(2,4)-\frac{4}{120}\cdot A_2(3,4)-\frac{4}{120}\cdot A_2(4,1)$$

$$-\frac{4}{120}\cdot A_2(4,2)-\frac{4}{120}\cdot A_2(4,3)-\frac{4}{120}\cdot A_2(4,4)-\frac{4}{120}\cdot A_3(1,1)$$

$$=\frac{0}{120\cdot 4(1/2)^3}+\frac{20}{120\cdot 5(1/2)^4}+\frac{4}{120}\cdot\frac{9334}{8640}+\frac{4}{120}\cdot\frac{9334}{8640}+\frac{4}{120}\cdot\frac{9334}{8640}+\frac{4}{120}\cdot\frac{9334}{8640}$$

$$+\frac{4}{120}\cdot\frac{9334}{8640}+\frac{4}{120}\cdot\frac{9334}{8640}-\frac{4}{120}\cdot\frac{31650}{8640}+\frac{4}{120}\cdot\frac{864}{8640}+\frac{4}{120}\cdot\frac{864}{8640}-\frac{4}{120}\cdot\frac{31650}{8640}$$

$$+\frac{4}{120}\cdot\frac{864}{8640}+\frac{4}{120}\cdot\frac{864}{8640}-\frac{4}{120}\cdot\frac{35976}{8640}-\frac{4}{120}\cdot\frac{40104}{8640}$$

$$=\frac{9}{40}.$$

$J_{14}$ : 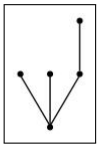

$$\frac{t_{\rm inj}(C_4,J_{14})}{4(1/2)^3}+\frac{t_{\rm inj}(C_5,\overline{J_{14}})}{5(1/2)^4}-\frac{2}{120}\cdot A_1(2,7)-\frac{2}{120}\cdot A_1(2,8)-\frac{2}{120}\cdot A_1(3,6)-\frac{2}{120}\cdot A_1(3,8)$$

$$-\frac{2}{120}\cdot A_1(4,5)-\frac{2}{120}\cdot A_1(4,8)-\frac{2}{120}\cdot A_1(5,4)-\frac{2}{120}\cdot A_1(6,3)-\frac{2}{120}\cdot A_1(7,2)-\frac{2}{120}\cdot A_1(8,2)$$

$$-\frac{2}{120}\cdot A_1(8,3)-\frac{2}{120}\cdot A_1(8,4)-\frac{2}{120}\cdot A_2(1,6)-\frac{2}{120}\cdot A_2(1,7)-\frac{2}{120}\cdot A_2(2,6)-\frac{2}{120}\cdot A_2(3,7)$$

$$-\frac{2}{120}\cdot A_2(6,1)-\frac{2}{120}\cdot A_2(6,2)-\frac{2}{120}\cdot A_2(7,1)-\frac{2}{120}\cdot A_2(7,3)-\frac{2}{120}\cdot A_3(1,2)-\frac{2}{120}\cdot A_3(2,1)$$

$$-\frac{2}{120}\cdot A_3(2,3)-\frac{2}{120}\cdot A_3(2,4)-\frac{2}{120}\cdot A_3(3,2)-\frac{2}{120}\cdot A_3(3,3)-\frac{2}{120}\cdot A_3(4,2)-\frac{2}{120}\cdot A_3(4,4)$$

$$=\frac{0}{120\cdot 4(1/2)^3}+\frac{0}{120\cdot 5(1/2)^4}+\frac{2}{120}\cdot\frac{9334}{8640}+\frac{2}{120}\cdot\frac{6786}{8640}+\frac{2}{120}\cdot\frac{9334}{8640}+\frac{2}{120}\cdot\frac{6786}{8640}$$

$$+\frac{2}{120}\cdot\frac{9334}{8640}+\frac{2}{120}\cdot\frac{6786}{8640}+\frac{2}{120}\cdot\frac{9334}{8640}+\frac{2}{120}\cdot\frac{9334}{8640}+\frac{2}{120}\cdot\frac{9334}{8640}+\frac{2}{120}\cdot\frac{6786}{8640}$$

$$+\frac{2}{120}\cdot\frac{6786}{8640}+\frac{2}{120}\cdot\frac{6786}{8640}+\frac{2}{120}\cdot\frac{7632}{8640}+\frac{2}{120}\cdot\frac{7632}{8640}+\frac{2}{120}\cdot\frac{5469}{8640}+\frac{2}{120}\cdot\frac{5469}{8640}$$

$$+\frac{2}{120}\cdot\frac{7632}{8640}+\frac{2}{120}\cdot\frac{5469}{8640}+\frac{2}{120}\cdot\frac{7632}{8640}+\frac{2}{120}\cdot\frac{5469}{8640}-\frac{2}{120}\cdot\frac{7458}{8640}-\frac{2}{120}\cdot\frac{7458}{8640}$$

$$+\frac{2}{120}\cdot\frac{3888}{8640}+\frac{2}{120}\cdot\frac{3888}{8640}+\frac{2}{120}\cdot\frac{3888}{8640}-\frac{2}{120}\cdot\frac{16560}{8640}+\frac{2}{120}\cdot\frac{3888}{8640}-\frac{2}{120}\cdot\frac{16560}{8640}$$

$$= \frac{9}{40}.$$

$J_{15}$ : 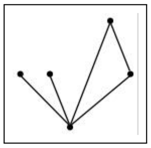

$$\frac{t_{\text{inj}}(C_4, J_{15})}{4(1/2)^3} + \frac{t_{\text{inj}}(C_5, \overline{J_{15}})}{5(1/2)^4} - \frac{4}{120} \cdot A_1(2,8) - \frac{4}{120} \cdot A_1(3,8) - \frac{4}{120} \cdot A_1(4,8) - \frac{4}{120} \cdot A_1(8,2)$$

$$- \frac{4}{120} \cdot A_1(8,3) - \frac{4}{120} \cdot A_1(8,4) - \frac{4}{120} \cdot A_2(1,8) - \frac{4}{120} \cdot A_2(8,1) - \frac{4}{120} \cdot A_3(2,2) - \frac{4}{120} \cdot A_3(2,5)$$
$$- \frac{4}{120} \cdot A_3(2,6) - \frac{4}{120} \cdot A_3(5,2) - \frac{4}{120} \cdot A_3(6,2) - \frac{4}{120} \cdot A_4(2,2) - \frac{4}{120} \cdot A_4(3,3) - \frac{4}{120} \cdot A_4(4,4)$$

$$= \frac{0}{120 \cdot 4(1/2)^3} + \frac{0}{120 \cdot 5(1/2)^4} + \frac{4}{120} \cdot \frac{6786}{8640} + \frac{4}{120} \cdot \frac{6786}{8640} + \frac{4}{120} \cdot \frac{6786}{8640} + \frac{4}{120} \cdot \frac{6786}{8640}$$
$$+ \frac{4}{120} \cdot \frac{6786}{8640} + \frac{4}{120} \cdot \frac{6786}{8640} + \frac{4}{120} \cdot \frac{43440}{8640} + \frac{4}{120} \cdot \frac{43440}{8640} - \frac{4}{120} \cdot \frac{33852}{8640} - \frac{4}{120} \cdot \frac{978}{8640}$$
$$- \frac{4}{120} \cdot \frac{978}{8640} - \frac{4}{120} \cdot \frac{978}{8640} - \frac{4}{120} \cdot \frac{978}{8640} - \frac{4}{120} \cdot \frac{10504}{8640} - \frac{4}{120} \cdot \frac{10504}{8640} - \frac{4}{120} \cdot \frac{10504}{8640}$$

$$= \frac{9}{40}.$$

$J_{16}$ : 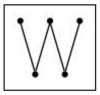

$$\frac{t_{\text{inj}}(C_4, J_{16})}{4(1/2)^3} + \frac{t_{\text{inj}}(C_5, \overline{J_{16}})}{5(1/2)^4} - \frac{2}{120} \cdot A_1(5,6) - \frac{2}{120} \cdot A_1(5,7) - \frac{2}{120} \cdot A_1(6,5) - \frac{2}{120} \cdot A_1(6,7)$$

$$- \frac{2}{120} \cdot A_1(7,5) - \frac{2}{120} \cdot A_1(7,6) - \frac{2}{120} \cdot A_2(2,4) - \frac{2}{120} \cdot A_2(2,7) - \frac{2}{120} \cdot A_2(3,4) - \frac{2}{120} \cdot A_2(3,6)$$
$$- \frac{2}{120} \cdot A_2(4,2) - \frac{2}{120} \cdot A_2(4,3) - \frac{2}{120} \cdot A_2(4,6) - \frac{2}{120} \cdot A_2(4,7) - \frac{2}{120} \cdot A_2(6,3) - \frac{2}{120} \cdot A_2(6,4)$$
$$- \frac{2}{120} \cdot A_2(7,2) - \frac{2}{120} \cdot A_2(7,4) - \frac{2}{120} \cdot A_3(1,3) - \frac{2}{120} \cdot A_3(1,4) - \frac{2}{120} \cdot A_3(3,1) - \frac{2}{120} \cdot A_3(3,4)$$
$$- \frac{2}{120} \cdot A_3(4,1) - \frac{2}{120} \cdot A_3(4,3)$$
$$= \frac{0}{120 \cdot 4(1/2)^3} + \frac{10}{120 \cdot 5(1/2)^4} + \frac{2}{120} \cdot \frac{720}{8640} + \frac{2}{120} \cdot \frac{720}{8640} + \frac{2}{120} \cdot \frac{720}{8640} + \frac{2}{120} \cdot \frac{720}{8640}$$

$$+\frac{2}{120}\cdot\frac{720}{8640}+\frac{2}{120}\cdot\frac{720}{8640}+\frac{2}{120}\cdot\frac{864}{8640}+\frac{2}{120}\cdot\frac{6120}{8640}+\frac{2}{120}\cdot\frac{864}{8640}+\frac{2}{120}\cdot\frac{6120}{8640}$$
$$+\frac{2}{120}\cdot\frac{864}{8640}+\frac{2}{120}\cdot\frac{864}{8640}+\frac{2}{120}\cdot\frac{111}{8640}+\frac{2}{120}\cdot\frac{111}{8640}+\frac{2}{120}\cdot\frac{6120}{8640}+\frac{2}{120}\cdot\frac{111}{8640}$$
$$+\frac{2}{120}\cdot\frac{6120}{8640}+\frac{2}{120}\cdot\frac{111}{8640}-\frac{2}{120}\cdot\frac{11880}{8640}-\frac{2}{120}\cdot\frac{11880}{8640}-\frac{2}{120}\cdot\frac{11880}{8640}-\frac{2}{120}\cdot\frac{3390}{8640}$$
$$-\frac{2}{120}\cdot\frac{11880}{8640}-\frac{2}{120}\cdot\frac{3390}{8640}$$
$$=\frac{9}{40}.$$

$J_{17}$ : 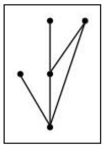

$$\frac{t_{\mathrm{inj}}(C_4,J_{17})}{4(1/2)^3}+\frac{t_{\mathrm{inj}}(C_5,\overline{J_{17}})}{5(1/2)^4}-\frac{2}{120}\cdot A_1(5,6)-\frac{2}{120}\cdot A_1(5,7)-\frac{2}{120}\cdot A_1(6,5)-\frac{2}{120}\cdot A_1(6,7)$$
$$-\frac{2}{120}\cdot A_1(7,5)-\frac{2}{120}\cdot A_1(7,6)-\frac{2}{120}\cdot A_2(2,6)-\frac{2}{120}\cdot A_2(2,8)-\frac{2}{120}\cdot A_2(3,7)-\frac{2}{120}\cdot A_2(3,8)$$
$$-\frac{2}{120}\cdot A_2(6,2)-\frac{2}{120}\cdot A_2(7,3)-\frac{2}{120}\cdot A_2(8,2)-\frac{2}{120}\cdot A_2(8,3)-\frac{2}{120}\cdot A_3(1,5)-\frac{2}{120}\cdot A_3(1,6)$$
$$-\frac{2}{120}\cdot A_3(3,5)-\frac{2}{120}\cdot A_3(4,6)-\frac{2}{120}\cdot A_3(5,1)-\frac{2}{120}\cdot A_3(5,3)-\frac{2}{120}\cdot A_3(6,1)-\frac{2}{120}\cdot A_3(6,4)$$
$$-\frac{2}{120}\cdot A_4(2,3)-\frac{2}{120}\cdot A_4(2,4)-\frac{2}{120}\cdot A_4(3,2)-\frac{2}{120}\cdot A_4(3,4)-\frac{2}{120}\cdot A_4(4,2)-\frac{2}{120}\cdot A_4(4,3)$$

$$=\frac{0}{120\cdot 4(1/2)^3}+\frac{0}{120\cdot 5(1/2)^4}+\frac{2}{120}\cdot\frac{720}{8640}+\frac{2}{120}\cdot\frac{720}{8640}+\frac{2}{120}\cdot\frac{720}{8640}+\frac{2}{120}\cdot\frac{720}{8640}$$
$$+\frac{2}{120}\cdot\frac{720}{8640}+\frac{2}{120}\cdot\frac{720}{8640}+\frac{2}{120}\cdot\frac{5469}{8640}+\frac{2}{120}\cdot\frac{6264}{8640}+\frac{2}{120}\cdot\frac{5469}{8640}+\frac{2}{120}\cdot\frac{6264}{8640}$$
$$+\frac{2}{120}\cdot\frac{5469}{8640}+\frac{2}{120}\cdot\frac{5469}{8640}+\frac{2}{120}\cdot\frac{6264}{8640}+\frac{2}{120}\cdot\frac{6264}{8640}+\frac{2}{120}\cdot\frac{10095}{8640}+\frac{2}{120}\cdot\frac{10095}{8640}$$
$$+\frac{2}{120}\cdot\frac{3660}{8640}+\frac{2}{120}\cdot\frac{3660}{8640}+\frac{2}{120}\cdot\frac{10095}{8640}+\frac{2}{120}\cdot\frac{3660}{8640}+\frac{2}{120}\cdot\frac{10095}{8640}+\frac{2}{120}\cdot\frac{3660}{8640}$$
$$+\frac{2}{120}\cdot\frac{1728}{8640}+\frac{2}{120}\cdot\frac{1728}{8640}+\frac{2}{120}\cdot\frac{1728}{8640}+\frac{2}{120}\cdot\frac{1728}{8640}+\frac{2}{120}\cdot\frac{1728}{8640}+\frac{2}{120}\cdot\frac{1728}{8640}$$

$$=\frac{9}{40}.$$

$J_{18}$ : 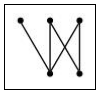

$$\frac{t_{\text{inj}}(C_4, J_{18})}{4(1/2)^3} + \frac{t_{\text{inj}}(C_5, \overline{J_{18}})}{5(1/2)^4} - \frac{2}{120} \cdot A_1(5,8) - \frac{2}{120} \cdot A_1(6,8) - \frac{2}{120} \cdot A_1(7,8) - \frac{2}{120} \cdot A_1(8,5)$$

$$- \frac{2}{120} \cdot A_1(8,6) - \frac{2}{120} \cdot A_1(8,7) - \frac{2}{120} \cdot A_2(2,7) - \frac{2}{120} \cdot A_2(3,6) - \frac{2}{120} \cdot A_2(6,3) - \frac{2}{120} \cdot A_2(6,6)$$
$$- \frac{2}{120} \cdot A_2(7,2) - \frac{2}{120} \cdot A_2(7,7) - \frac{2}{120} \cdot A_3(1,7) - \frac{2}{120} \cdot A_3(2,3) - \frac{2}{120} \cdot A_3(2,4) - \frac{2}{120} \cdot A_3(2,7)$$
$$- \frac{2}{120} \cdot A_3(3,2) - \frac{2}{120} \cdot A_3(3,7) - \frac{2}{120} \cdot A_3(4,2) - \frac{2}{120} \cdot A_3(4,7) - \frac{2}{120} \cdot A_3(7,1) - \frac{2}{120} \cdot A_3(7,2)$$
$$- \frac{2}{120} \cdot A_3(7,3) - \frac{2}{120} \cdot A_3(7,4)$$
$$= \frac{8}{120 \cdot 4(1/2)^3} + \frac{0}{120 \cdot 5(1/2)^4} - \frac{2}{120} \cdot \frac{6620}{8640} - \frac{2}{120} \cdot \frac{6620}{8640} - \frac{2}{120} \cdot \frac{6620}{8640} - \frac{2}{120} \cdot \frac{6620}{8640}$$
$$- \frac{2}{120} \cdot \frac{6620}{8640} - \frac{2}{120} \cdot \frac{6620}{8640} + \frac{2}{120} \cdot \frac{6120}{8640} + \frac{2}{120} \cdot \frac{6120}{8640} + \frac{2}{120} \cdot \frac{6120}{8640} - \frac{2}{120} \cdot \frac{14586}{8640}$$
$$+ \frac{2}{120} \cdot \frac{6120}{8640} - \frac{2}{120} \cdot \frac{14586}{8640} + \frac{2}{120} \cdot \frac{17496}{8640} + \frac{2}{120} \cdot \frac{3888}{8640} + \frac{2}{120} \cdot \frac{3888}{8640} + \frac{2}{120} \cdot \frac{15768}{8640}$$
$$+ \frac{2}{120} \cdot \frac{3888}{8640} + \frac{2}{120} \cdot \frac{2463}{8640} + \frac{2}{120} \cdot \frac{3888}{8640} + \frac{2}{120} \cdot \frac{2463}{8640} + \frac{2}{120} \cdot \frac{17496}{8640} + \frac{2}{120} \cdot \frac{15768}{8640}$$
$$+ \frac{2}{120} \cdot \frac{2463}{8640} + \frac{2}{120} \cdot \frac{2463}{8640}$$
$$= \frac{9}{40}.$$

$J_{19}$ : 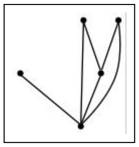

$$\frac{t_{\text{inj}}(C_4, J_{19})}{4(1/2)^3} + \frac{t_{\text{inj}}(C_5, \overline{J_{19}})}{5(1/2)^4} - \frac{2}{120} \cdot A_1(5,8) - \frac{2}{120} \cdot A_1(6,8) - \frac{2}{120} \cdot A_1(7,8) - \frac{2}{120} \cdot A_1(8,5)$$

$$- \frac{2}{120} \cdot A_1(8,6) - \frac{2}{120} \cdot A_1(8,7) - \frac{2}{120} \cdot A_2(2,8) - \frac{2}{120} \cdot A_2(3,8) - \frac{2}{120} \cdot A_2(8,2) - \frac{2}{120} \cdot A_2(8,3)$$
$$- \frac{2}{120} \cdot A_3(1,8) - \frac{2}{120} \cdot A_3(2,5) - \frac{2}{120} \cdot A_3(2,6) - \frac{2}{120} \cdot A_3(2,8) - \frac{2}{120} \cdot A_3(5,2) - \frac{2}{120} \cdot A_3(5,5)$$
$$- \frac{2}{120} \cdot A_3(6,2) - \frac{2}{120} \cdot A_3(6,6) - \frac{2}{120} \cdot A_3(8,1) - \frac{2}{120} \cdot A_3(8,2) - \frac{2}{120} \cdot A_4(2,5) - \frac{2}{120} \cdot A_4(2,6)$$

$$-\frac{2}{120}\cdot A_4(3,5)-\frac{2}{120}\cdot A_4(3,7)-\frac{2}{120}\cdot A_4(4,6)-\frac{2}{120}\cdot A_4(4,7)-\frac{2}{120}\cdot A_4(5,2)-\frac{2}{120}\cdot A_4(5,3)$$
$$-\frac{2}{120}\cdot A_4(6,2)-\frac{2}{120}\cdot A_4(6,4)-\frac{2}{120}\cdot A_4(7,3)-\frac{2}{120}\cdot A_4(7,4)$$
$$=\frac{8}{120\cdot 4(1/2)^3}+\frac{0}{120\cdot 5(1/2)^4}-\frac{2}{120}\cdot\frac{6620}{8640}-\frac{2}{120}\cdot\frac{6620}{8640}-\frac{2}{120}\cdot\frac{6620}{8640}-\frac{2}{120}\cdot\frac{6620}{8640}$$
$$-\frac{2}{120}\cdot\frac{6620}{8640}-\frac{2}{120}\cdot\frac{6620}{8640}+\frac{2}{120}\cdot\frac{6264}{8640}+\frac{2}{120}\cdot\frac{6264}{8640}+\frac{2}{120}\cdot\frac{6264}{8640}+\frac{2}{120}\cdot\frac{6264}{8640}$$
$$+\frac{2}{120}\cdot\frac{33636}{8640}-\frac{2}{120}\cdot\frac{978}{8640}-\frac{2}{120}\cdot\frac{978}{8640}+\frac{2}{120}\cdot\frac{19722}{8640}-\frac{2}{120}\cdot\frac{978}{8640}-\frac{2}{120}\cdot\frac{15366}{8640}$$
$$-\frac{2}{120}\cdot\frac{978}{8640}-\frac{2}{120}\cdot\frac{15366}{8640}+\frac{2}{120}\cdot\frac{33636}{8640}+\frac{2}{120}\cdot\frac{19722}{8640}-\frac{2}{120}\cdot\frac{824}{8640}-\frac{2}{120}\cdot\frac{824}{8640}$$
$$-\frac{2}{120}\cdot\frac{824}{8640}-\frac{2}{120}\cdot\frac{824}{8640}-\frac{2}{120}\cdot\frac{824}{8640}-\frac{2}{120}\cdot\frac{824}{8640}-\frac{2}{120}\cdot\frac{824}{8640}-\frac{2}{120}\cdot\frac{824}{8640}$$
$$-\frac{2}{120}\cdot\frac{824}{8640}-\frac{2}{120}\cdot\frac{824}{8640}-\frac{2}{120}\cdot\frac{824}{8640}-\frac{2}{120}\cdot\frac{824}{8640}$$
$$=\frac{9}{40}.$$

$J_{20}$ : 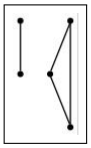

$$\frac{t_{\text{inj}}(C_4,J_{20})}{4(1/2)^3}+\frac{t_{\text{inj}}(C_5,\overline{J_{20}})}{5(1/2)^4}-\frac{12}{120}\cdot A_2(4,4)-\frac{12}{120}\cdot A_2(4,5)-\frac{12}{120}\cdot A_2(5,4)-\frac{12}{120}\cdot A_4(1,1)$$
$$=\frac{0}{120\cdot 4(1/2)^3}+\frac{0}{120\cdot 5(1/2)^4}-\frac{12}{120}\cdot\frac{35976}{8640}+\frac{12}{120}\cdot\frac{35484}{8640}+\frac{12}{120}\cdot\frac{35484}{8640}-\frac{12}{120}\cdot\frac{15552}{8640}$$
$$=\frac{9}{40}.$$

$J_{21}$ : 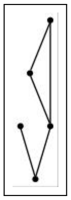

$$\frac{t_{\text{inj}}(C_4,J_{21})}{4(1/2)^3}+\frac{t_{\text{inj}}(C_5,\overline{J_{21}})}{5(1/2)^4}-\frac{2}{120}\cdot A_2(4,5)-\frac{2}{120}\cdot A_2(4,6)-\frac{2}{120}\cdot A_2(4,7)-\frac{2}{120}\cdot A_2(4,8)$$

$$-\frac{2}{120}\cdot A_2(5,4)-\frac{2}{120}\cdot A_2(5,6)-\frac{2}{120}\cdot A_2(5,7)-\frac{2}{120}\cdot A_2(6,4)-\frac{2}{120}\cdot A_2(6,5)-\frac{2}{120}\cdot A_2(7,4)$$
$$-\frac{2}{120}\cdot A_2(7,5)-\frac{2}{120}\cdot A_2(8,4)-\frac{2}{120}\cdot A_3(3,3)-\frac{2}{120}\cdot A_3(3,6)-\frac{2}{120}\cdot A_3(4,4)-\frac{2}{120}\cdot A_3(4,5)$$
$$-\frac{2}{120}\cdot A_3(5,4)-\frac{2}{120}\cdot A_3(6,3)-\frac{2}{120}\cdot A_4(1,2)-\frac{2}{120}\cdot A_4(1,3)-\frac{2}{120}\cdot A_4(1,4)-\frac{2}{120}\cdot A_4(2,1)$$
$$-\frac{2}{120}\cdot A_4(3,1)-\frac{2}{120}\cdot A_4(4,1)$$
$$=\frac{0}{120\cdot 4(1/2)^3}+\frac{0}{120\cdot 5(1/2)^4}+\frac{2}{120}\cdot\frac{35484}{8640}+\frac{2}{120}\cdot\frac{111}{8640}+\frac{2}{120}\cdot\frac{111}{8640}+\frac{2}{120}\cdot\frac{30192}{8640}$$
$$+\frac{2}{120}\cdot\frac{35484}{8640}-\frac{2}{120}\cdot\frac{216}{8640}-\frac{2}{120}\cdot\frac{216}{8640}+\frac{2}{120}\cdot\frac{111}{8640}-\frac{2}{120}\cdot\frac{216}{8640}+\frac{2}{120}\cdot\frac{111}{8640}$$
$$-\frac{2}{120}\cdot\frac{216}{8640}+\frac{2}{120}\cdot\frac{30192}{8640}-\frac{2}{120}\cdot\frac{16560}{8640}+\frac{2}{120}\cdot\frac{12075}{8640}-\frac{2}{120}\cdot\frac{16560}{8640}+\frac{2}{120}\cdot\frac{12075}{8640}$$
$$+\frac{2}{120}\cdot\frac{12075}{8640}+\frac{2}{120}\cdot\frac{12075}{8640}-\frac{2}{120}\cdot\frac{4912}{8640}-\frac{2}{120}\cdot\frac{4912}{8640}-\frac{2}{120}\cdot\frac{4912}{8640}-\frac{2}{120}\cdot\frac{4912}{8640}$$
$$-\frac{2}{120}\cdot\frac{4912}{8640}-\frac{2}{120}\cdot\frac{4912}{8640}$$
$$=\frac{9}{40}.$$

$J_{22}$ : 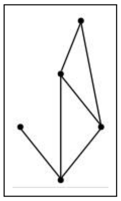

$$\frac{t_{\rm inj}(C_4,J_{22})}{4(1/2)^3}+\frac{t_{\rm inj}(C_5,\overline{J_{22}})}{5(1/2)^4}-\frac{2}{120}\cdot A_2(5,6)-\frac{2}{120}\cdot A_2(5,7)-\frac{2}{120}\cdot A_2(5,8)-\frac{2}{120}\cdot A_2(6,5)$$
$$-\frac{2}{120}\cdot A_2(6,6)-\frac{2}{120}\cdot A_2(7,5)-\frac{2}{120}\cdot A_2(7,7)-\frac{2}{120}\cdot A_2(8,5)-\frac{2}{120}\cdot A_3(3,5)-\frac{2}{120}\cdot A_3(3,8)$$
$$-\frac{2}{120}\cdot A_3(4,6)-\frac{2}{120}\cdot A_3(4,8)-\frac{2}{120}\cdot A_3(5,3)-\frac{2}{120}\cdot A_3(6,4)-\frac{2}{120}\cdot A_3(8,3)-\frac{2}{120}\cdot A_3(8,4)$$
$$-\frac{2}{120}\cdot A_4(1,5)-\frac{2}{120}\cdot A_4(1,6)-\frac{2}{120}\cdot A_4(1,7)-\frac{2}{120}\cdot A_4(2,7)-\frac{2}{120}\cdot A_4(3,6)-\frac{2}{120}\cdot A_4(4,5)$$
$$-\frac{2}{120}\cdot A_4(5,1)-\frac{2}{120}\cdot A_4(5,4)-\frac{2}{120}\cdot A_4(6,1)-\frac{2}{120}\cdot A_4(6,3)-\frac{2}{120}\cdot A_4(7,1)-\frac{2}{120}\cdot A_4(7,2)$$
$$=\frac{8}{120\cdot 4(1/2)^3}+\frac{0}{120\cdot 5(1/2)^4}-\frac{2}{120}\cdot\frac{216}{8640}-\frac{2}{120}\cdot\frac{216}{8640}-\frac{2}{120}\cdot\frac{29448}{8640}-\frac{2}{120}\cdot\frac{216}{8640}$$

$$-\frac{2}{120}\cdot\frac{14586}{8640}-\frac{2}{120}\cdot\frac{216}{8640}-\frac{2}{120}\cdot\frac{14586}{8640}-\frac{2}{120}\cdot\frac{29448}{8640}+\frac{2}{120}\cdot\frac{3660}{8640}+\frac{2}{120}\cdot\frac{9744}{8640}$$
$$+\frac{2}{120}\cdot\frac{3660}{8640}+\frac{2}{120}\cdot\frac{9744}{8640}+\frac{2}{120}\cdot\frac{3660}{8640}+\frac{2}{120}\cdot\frac{3660}{8640}+\frac{2}{120}\cdot\frac{9744}{8640}+\frac{2}{120}\cdot\frac{9744}{8640}$$
$$+\frac{2}{120}\cdot\frac{5166}{8640}+\frac{2}{120}\cdot\frac{5166}{8640}+\frac{2}{120}\cdot\frac{5166}{8640}+\frac{2}{120}\cdot\frac{8640}{8640}+\frac{2}{120}\cdot\frac{8640}{8640}+\frac{2}{120}\cdot\frac{8640}{8640}$$
$$+\frac{2}{120}\cdot\frac{5166}{8640}+\frac{2}{120}\cdot\frac{8640}{8640}+\frac{2}{120}\cdot\frac{5166}{8640}+\frac{2}{120}\cdot\frac{8640}{8640}+\frac{2}{120}\cdot\frac{5166}{8640}+\frac{2}{120}\cdot\frac{8640}{8640}$$

$$=\frac{9}{40}.$$

$J_{23}$ : 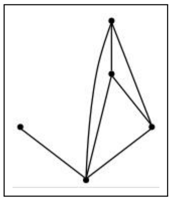

$$\frac{t_{\text{inj}}(C_4,J_{23})}{4(1/2)^3}+\frac{t_{\text{inj}}(C_5,\overline{J_{23}})}{5(1/2)^4}-\frac{6}{120}\cdot A_2(5,8)-\frac{6}{120}\cdot A_2(8,5)-\frac{6}{120}\cdot A_3(5,5)-\frac{6}{120}\cdot A_3(6,6)$$
$$-\frac{6}{120}\cdot A_4(1,8)-\frac{6}{120}\cdot A_4(2,8)-\frac{6}{120}\cdot A_4(3,8)-\frac{6}{120}\cdot A_4(4,8)-\frac{6}{120}\cdot A_4(8,1)-\frac{6}{120}\cdot A_4(8,2)$$
$$-\frac{6}{120}\cdot A_4(8,3)-\frac{6}{120}\cdot A_4(8,4)$$
$$=\frac{24}{120\cdot 4(1/2)^3}+\frac{0}{120\cdot 5(1/2)^4}-\frac{6}{120}\cdot\frac{29448}{8640}-\frac{6}{120}\cdot\frac{29448}{8640}-\frac{6}{120}\cdot\frac{15366}{8640}-\frac{6}{120}\cdot\frac{15366}{8640}$$
$$+\frac{6}{120}\cdot\frac{14790}{8640}+\frac{6}{120}\cdot\frac{4968}{8640}+\frac{6}{120}\cdot\frac{4968}{8640}+\frac{6}{120}\cdot\frac{4968}{8640}+\frac{6}{120}\cdot\frac{14790}{8640}+\frac{6}{120}\cdot\frac{4968}{8640}$$
$$+\frac{6}{120}\cdot\frac{4968}{8640}+\frac{6}{120}\cdot\frac{4968}{8640}$$
$$=\frac{9}{40}.$$

$J_{24}$ : 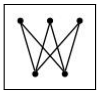

$$\frac{t_{\text{inj}}(C_4,J_{24})}{4(1/2)^3}+\frac{t_{\text{inj}}(C_5,\overline{J_{24}})}{5(1/2)^4}-\frac{12}{120}\cdot A_1(8,8)-\frac{12}{120}\cdot A_3(2,7)-\frac{12}{120}\cdot A_3(7,2)-\frac{12}{120}\cdot A_3(7,7)$$

$$= \frac{24}{120 \cdot 4(1/2)^3} + \frac{0}{120 \cdot 5(1/2)^4} - \frac{12}{120} \cdot \frac{22284}{8640} + \frac{12}{120} \cdot \frac{15768}{8640} + \frac{12}{120} \cdot \frac{15768}{8640} - \frac{12}{120} \cdot \frac{24372}{8640}$$

$$= \frac{9}{40}.$$

$J_{25}$ : 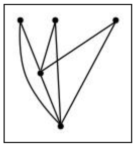

$$\frac{t_{\text{inj}}(C_4, J_{25})}{4(1/2)^3} + \frac{t_{\text{inj}}(C_5, \overline{J_{25}})}{5(1/2)^4} - \frac{12}{120} \cdot A_1(8,8) - \frac{12}{120} \cdot A_3(2,8) - \frac{12}{120} \cdot A_3(8,2) - \frac{12}{120} \cdot A_4(5,5)$$

$$- \frac{12}{120} \cdot A_4(6,6) - \frac{12}{120} \cdot A_4(7,7)$$

$$= \frac{24}{120 \cdot 4(1/2)^3} + \frac{0}{120 \cdot 5(1/2)^4} - \frac{12}{120} \cdot \frac{22284}{8640} + \frac{12}{120} \cdot \frac{19722}{8640} + \frac{12}{120} \cdot \frac{19722}{8640} - \frac{12}{120} \cdot \frac{10760}{8640}$$

$$- \frac{12}{120} \cdot \frac{10760}{8640} - \frac{12}{120} \cdot \frac{10760}{8640}$$

$$= \frac{9}{40}.$$

$J_{26}$ : 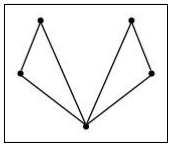

$$\frac{t_{\text{inj}}(C_4, J_{26})}{4(1/2)^3} + \frac{t_{\text{inj}}(C_5, \overline{J_{26}})}{5(1/2)^4} - \frac{8}{120} \cdot A_2(4,8) - \frac{8}{120} \cdot A_2(8,4) - \frac{8}{120} \cdot A_3(5,6) - \frac{8}{120} \cdot A_3(6,5)$$

$$- \frac{8}{120} \cdot A_4(2,2) - \frac{8}{120} \cdot A_4(3,3) - \frac{8}{120} \cdot A_4(4,4)$$

$$= \frac{0}{120 \cdot 4(1/2)^3} + \frac{0}{120 \cdot 5(1/2)^4} + \frac{8}{120} \cdot \frac{30192}{8640} + \frac{8}{120} \cdot \frac{30192}{8640} + \frac{8}{120} \cdot \frac{144}{8640} + \frac{8}{120} \cdot \frac{144}{8640}$$

$$- \frac{8}{120} \cdot \frac{10504}{8640} - \frac{8}{120} \cdot \frac{10504}{8640} - \frac{8}{120} \cdot \frac{10504}{8640}$$

$$= \frac{9}{40}.$$

$J_{27}$ : 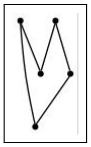

$$\frac{t_{\text{inj}}(C_4, J_{27})}{4(1/2)^3} + \frac{t_{\text{inj}}(C_5, \overline{J_{27}})}{5(1/2)^4} - \frac{10}{120} \cdot A_2(6,7) - \frac{10}{120} \cdot A_2(7,6) - \frac{10}{120} \cdot A_3(3,4) - \frac{10}{120} \cdot A_3(4,3)$$

$$= \frac{0}{120 \cdot 4(1/2)^3} + \frac{10}{120 \cdot 5(1/2)^4} + \frac{10}{120} \cdot \frac{1230}{8640} + \frac{10}{120} \cdot \frac{1230}{8640} - \frac{10}{120} \cdot \frac{3390}{8640} - \frac{10}{120} \cdot \frac{3390}{8640}$$

$$= \frac{9}{40}.$$

$J_{28}$ : 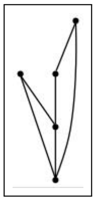

$$\frac{t_{\text{inj}}(C_4, J_{28})}{4(1/2)^3} + \frac{t_{\text{inj}}(C_5, \overline{J_{28}})}{5(1/2)^4} - \frac{2}{120} \cdot A_2(6,7) - \frac{2}{120} \cdot A_2(6,8) - \frac{2}{120} \cdot A_2(7,6) - \frac{2}{120} \cdot A_2(7,8)$$

$$- \frac{2}{120} \cdot A_2(8,6) - \frac{2}{120} \cdot A_2(8,7) - \frac{2}{120} \cdot A_3(3,6) - \frac{2}{120} \cdot A_3(3,7) - \frac{2}{120} \cdot A_3(4,5) - \frac{2}{120} \cdot A_3(4,7)$$

$$- \frac{2}{120} \cdot A_3(5,4) - \frac{2}{120} \cdot A_3(5,7) - \frac{2}{120} \cdot A_3(6,3) - \frac{2}{120} \cdot A_3(6,7) - \frac{2}{120} \cdot A_3(7,3) - \frac{2}{120} \cdot A_3(7,4)$$

$$- \frac{2}{120} \cdot A_3(7,5) - \frac{2}{120} \cdot A_3(7,6) - \frac{2}{120} \cdot A_4(2,3) - \frac{2}{120} \cdot A_4(2,4) - \frac{2}{120} \cdot A_4(3,2) - \frac{2}{120} \cdot A_4(3,4)$$

$$- \frac{2}{120} \cdot A_4(4,2) - \frac{2}{120} \cdot A_4(4,3)$$

$$= \frac{8}{120 \cdot 4(1/2)^3} + \frac{0}{120 \cdot 5(1/2)^4} + \frac{2}{120} \cdot \frac{1230}{8640} - \frac{2}{120} \cdot \frac{5760}{8640} + \frac{2}{120} \cdot \frac{1230}{8640} - \frac{2}{120} \cdot \frac{5760}{8640}$$

$$- \frac{2}{120} \cdot \frac{5760}{8640} - \frac{2}{120} \cdot \frac{5760}{8640} + \frac{2}{120} \cdot \frac{12075}{8640} + \frac{2}{120} \cdot \frac{2463}{8640} + \frac{2}{120} \cdot \frac{12075}{8640} + \frac{2}{120} \cdot \frac{2463}{8640}$$

$$+ \frac{2}{120} \cdot \frac{12075}{8640} - \frac{2}{120} \cdot \frac{105}{8640} + \frac{2}{120} \cdot \frac{12075}{8640} - \frac{2}{120} \cdot \frac{105}{8640} + \frac{2}{120} \cdot \frac{2463}{8640} + \frac{2}{120} \cdot \frac{2463}{8640}$$

$$- \frac{2}{120} \cdot \frac{105}{8640} - \frac{2}{120} \cdot \frac{105}{8640} + \frac{2}{120} \cdot \frac{1728}{8640} + \frac{2}{120} \cdot \frac{1728}{8640} + \frac{2}{120} \cdot \frac{1728}{8640} + \frac{2}{120} \cdot \frac{1728}{8640}$$

$$+ \frac{2}{120} \cdot \frac{1728}{8640} + \frac{2}{120} \cdot \frac{1728}{8640}$$

$$= \frac{9}{40}.$$

$J_{29}$ : 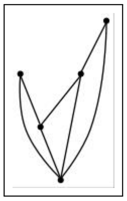

$$\frac{t_{\text{inj}}(C_4, J_{29})}{4(1/2)^3} + \frac{t_{\text{inj}}(C_5, \overline{J_{29}})}{5(1/2)^4} - \frac{2}{120} \cdot A_2(6,8) - \frac{2}{120} \cdot A_2(7,8) - \frac{2}{120} \cdot A_2(8,6) - \frac{2}{120} \cdot A_2(8,7)$$
$$-\frac{2}{120} \cdot A_3(3,8) - \frac{2}{120} \cdot A_3(4,8) - \frac{2}{120} \cdot A_3(5,6) - \frac{2}{120} \cdot A_3(5,8) - \frac{2}{120} \cdot A_3(6,5) - \frac{2}{120} \cdot A_3(6,8)$$
$$-\frac{2}{120} \cdot A_3(8,3) - \frac{2}{120} \cdot A_3(8,4) - \frac{2}{120} \cdot A_3(8,5) - \frac{2}{120} \cdot A_3(8,6) - \frac{2}{120} \cdot A_4(2,5) - \frac{2}{120} \cdot A_4(2,6)$$
$$-\frac{2}{120} \cdot A_4(3,5) - \frac{2}{120} \cdot A_4(3,7) - \frac{2}{120} \cdot A_4(4,6) - \frac{2}{120} \cdot A_4(4,7) - \frac{2}{120} \cdot A_4(5,2) - \frac{2}{120} \cdot A_4(5,3)$$
$$-\frac{2}{120} \cdot A_4(5,6) - \frac{2}{120} \cdot A_4(5,7) - \frac{2}{120} \cdot A_4(6,2) - \frac{2}{120} \cdot A_4(6,4) - \frac{2}{120} \cdot A_4(6,5) - \frac{2}{120} \cdot A_4(6,7)$$
$$-\frac{2}{120} \cdot A_4(7,3) - \frac{2}{120} \cdot A_4(7,4) - \frac{2}{120} \cdot A_4(7,5) - \frac{2}{120} \cdot A_4(7,6)$$
$$= \frac{16}{120 \cdot 4(1/2)^3} + \frac{0}{120 \cdot 5(1/2)^4} - \frac{2}{120} \cdot \frac{5760}{8640} - \frac{2}{120} \cdot \frac{5760}{8640} - \frac{2}{120} \cdot \frac{5760}{8640} - \frac{2}{120} \cdot \frac{5760}{8640}$$
$$+\frac{2}{120} \cdot \frac{9744}{8640} + \frac{2}{120} \cdot \frac{9744}{8640} + \frac{2}{120} \cdot \frac{144}{8640} - \frac{2}{120} \cdot \frac{9525}{8640} + \frac{2}{120} \cdot \frac{144}{8640} - \frac{2}{120} \cdot \frac{9525}{8640}$$
$$+\frac{2}{120} \cdot \frac{9744}{8640} + \frac{2}{120} \cdot \frac{9744}{8640} - \frac{2}{120} \cdot \frac{9525}{8640} - \frac{2}{120} \cdot \frac{9525}{8640} - \frac{2}{120} \cdot \frac{824}{8640} - \frac{2}{120} \cdot \frac{824}{8640}$$
$$-\frac{2}{120} \cdot \frac{824}{8640} - \frac{2}{120} \cdot \frac{824}{8640} - \frac{2}{120} \cdot \frac{824}{8640} - \frac{2}{120} \cdot \frac{824}{8640} - \frac{2}{120} \cdot \frac{824}{8640} - \frac{2}{120} \cdot \frac{824}{8640}$$
$$+\frac{2}{120} \cdot \frac{1694}{8640} + \frac{2}{120} \cdot \frac{1694}{8640} - \frac{2}{120} \cdot \frac{824}{8640} - \frac{2}{120} \cdot \frac{824}{8640} + \frac{2}{120} \cdot \frac{1694}{8640} + \frac{2}{120} \cdot \frac{1694}{8640}$$
$$-\frac{2}{120} \cdot \frac{824}{8640} - \frac{2}{120} \cdot \frac{824}{8640} + \frac{2}{120} \cdot \frac{1694}{8640} + \frac{2}{120} \cdot \frac{1694}{8640}$$
$$= \frac{9}{40}.$$

$J_{30}$ : 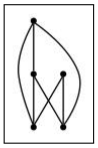

$$\frac{t_{\text{inj}}(C_4, J_{30})}{4(1/2)^3} + \frac{t_{\text{inj}}(C_5, \overline{J_{30}})}{5(1/2)^4} - \frac{4}{120} \cdot A_2(8,8) - \frac{4}{120} \cdot A_3(5,7) - \frac{4}{120} \cdot A_3(6,7) - \frac{4}{120} \cdot A_3(7,5)$$

$$-\frac{4}{120}\cdot A_3(7,6)-\frac{4}{120}\cdot A_3(7,7)-\frac{4}{120}\cdot A_3(7,8)-\frac{4}{120}\cdot A_3(8,7)-\frac{4}{120}\cdot A_4(2,7)-\frac{4}{120}\cdot A_4(3,6)$$
$$-\frac{4}{120}\cdot A_4(4,5)-\frac{4}{120}\cdot A_4(5,4)-\frac{4}{120}\cdot A_4(6,3)-\frac{4}{120}\cdot A_4(7,2)$$
$$=\frac{24}{120\cdot 4(1/2)^3}+\frac{0}{120\cdot 5(1/2)^4}-\frac{4}{120}\cdot\frac{45192}{8640}-\frac{4}{120}\cdot\frac{105}{8640}-\frac{4}{120}\cdot\frac{105}{8640}-\frac{4}{120}\cdot\frac{105}{8640}$$
$$-\frac{4}{120}\cdot\frac{105}{8640}-\frac{4}{120}\cdot\frac{24372}{8640}-\frac{4}{120}\cdot\frac{13608}{8640}-\frac{4}{120}\cdot\frac{13608}{8640}+\frac{4}{120}\cdot\frac{8640}{8640}+\frac{4}{120}\cdot\frac{8640}{8640}$$
$$+\frac{4}{120}\cdot\frac{8640}{8640}+\frac{4}{120}\cdot\frac{8640}{8640}+\frac{4}{120}\cdot\frac{8640}{8640}+\frac{4}{120}\cdot\frac{8640}{8640}$$
$$=\frac{9}{40}.$$

$J_{31}$ : 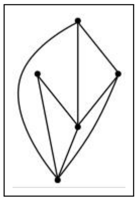

$$\frac{t_{\text{inj}}(C_4,J_{31})}{4(1/2)^3}+\frac{t_{\text{inj}}(C_5,\overline{J_{31}})}{5(1/2)^4}-\frac{4}{120}\cdot A_2(8,8)-\frac{4}{120}\cdot A_3(5,8)-\frac{4}{120}\cdot A_3(6,8)-\frac{4}{120}\cdot A_3(8,5)$$
$$-\frac{4}{120}\cdot A_3(8,6)-\frac{4}{120}\cdot A_4(2,8)-\frac{4}{120}\cdot A_4(3,8)-\frac{4}{120}\cdot A_4(4,8)-\frac{4}{120}\cdot A_4(5,5)-\frac{4}{120}\cdot A_4(5,8)$$
$$-\frac{4}{120}\cdot A_4(6,6)-\frac{4}{120}\cdot A_4(6,8)-\frac{4}{120}\cdot A_4(7,7)-\frac{4}{120}\cdot A_4(7,8)-\frac{4}{120}\cdot A_4(8,2)-\frac{4}{120}\cdot A_4(8,3)$$
$$-\frac{4}{120}\cdot A_4(8,4)-\frac{4}{120}\cdot A_4(8,5)-\frac{4}{120}\cdot A_4(8,6)-\frac{4}{120}\cdot A_4(8,7)$$
$$=\frac{40}{120\cdot 4(1/2)^3}+\frac{0}{120\cdot 5(1/2)^4}-\frac{4}{120}\cdot\frac{45192}{8640}-\frac{4}{120}\cdot\frac{9525}{8640}-\frac{4}{120}\cdot\frac{9525}{8640}-\frac{4}{120}\cdot\frac{9525}{8640}$$
$$-\frac{4}{120}\cdot\frac{9525}{8640}+\frac{4}{120}\cdot\frac{4968}{8640}+\frac{4}{120}\cdot\frac{4968}{8640}+\frac{4}{120}\cdot\frac{4968}{8640}-\frac{4}{120}\cdot\frac{10760}{8640}-\frac{4}{120}\cdot\frac{4786}{8640}$$
$$-\frac{4}{120}\cdot\frac{10760}{8640}-\frac{4}{120}\cdot\frac{4786}{8640}-\frac{4}{120}\cdot\frac{10760}{8640}-\frac{4}{120}\cdot\frac{4786}{8640}+\frac{4}{120}\cdot\frac{4968}{8640}+\frac{4}{120}\cdot\frac{4968}{8640}$$
$$+\frac{4}{120}\cdot\frac{4968}{8640}-\frac{4}{120}\cdot\frac{4786}{8640}-\frac{4}{120}\cdot\frac{4786}{8640}-\frac{4}{120}\cdot\frac{4786}{8640}$$
$$=\frac{9}{40}.$$

$J_{32}$ : 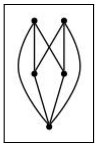

$$\frac{t_{\rm inj}(C_4,J_{32})}{4(1/2)^3}+\frac{t_{\rm inj}(C_5,\overline{J_{32}})}{5(1/2)^4}-\frac{8}{120}\cdot A_3(7,8)-\frac{8}{120}\cdot A_3(8,7)-\frac{8}{120}\cdot A_3(8,8)-\frac{8}{120}\cdot A_4(5,6)$$
$$-\frac{8}{120}\cdot A_4(5,7)-\frac{8}{120}\cdot A_4(6,5)-\frac{8}{120}\cdot A_4(6,7)-\frac{8}{120}\cdot A_4(7,5)-\frac{8}{120}\cdot A_4(7,6)$$
$$=\frac{40}{120\cdot 4(1/2)^3}+\frac{0}{120\cdot 5(1/2)^4}-\frac{8}{120}\cdot\frac{13608}{8640}-\frac{8}{120}\cdot\frac{13608}{8640}-\frac{8}{120}\cdot\frac{40188}{8640}+\frac{8}{120}\cdot\frac{1694}{8640}$$
$$+\frac{8}{120}\cdot\frac{1694}{8640}+\frac{8}{120}\cdot\frac{1694}{8640}+\frac{8}{120}\cdot\frac{1694}{8640}+\frac{8}{120}\cdot\frac{1694}{8640}+\frac{8}{120}\cdot\frac{1694}{8640}$$
$$=\frac{9}{40}.$$

$J_{33}$ : 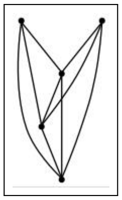

$$\frac{t_{\rm inj}(C_4,J_{33})}{4(1/2)^3}+\frac{t_{\rm inj}(C_5,\overline{J_{33}})}{5(1/2)^4}-\frac{12}{120}\cdot A_3(8,8)-\frac{12}{120}\cdot A_4(5,8)-\frac{12}{120}\cdot A_4(6,8)-\frac{12}{120}\cdot A_4(7,8)$$
$$-\frac{12}{120}\cdot A_4(8,5)-\frac{12}{120}\cdot A_4(8,6)-\frac{12}{120}\cdot A_4(8,7)-\frac{12}{120}\cdot A_4(8,8)$$
$$=\frac{72}{120\cdot 4(1/2)^3}+\frac{0}{120\cdot 5(1/2)^4}-\frac{12}{120}\cdot\frac{40188}{8640}-\frac{12}{120}\cdot\frac{4786}{8640}-\frac{12}{120}\cdot\frac{4786}{8640}-\frac{12}{120}\cdot\frac{4786}{8640}$$
$$-\frac{12}{120}\cdot\frac{4786}{8640}-\frac{12}{120}\cdot\frac{4786}{8640}-\frac{12}{120}\cdot\frac{4786}{8640}-\frac{12}{120}\cdot\frac{15336}{8640}$$
$$=\frac{9}{40}.$$

$J_{34}$ : 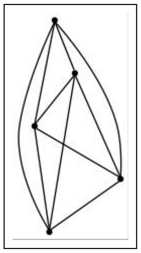

$$\frac{t_{\rm inj}(C_4,J_{34})}{4(1/2)^3}+\frac{t_{\rm inj}(C_5,\overline{J_{34}})}{5(1/2)^4}-\frac{120}{120}\cdot A_4(8,8)$$

$$= \frac{120}{120 \cdot 4(1/2)^3} + \frac{0}{120 \cdot 5(1/2)^4} - \frac{120}{120} \cdot \frac{15336}{8640}$$

$$= \frac{9}{40}.$$

# B Verification of Flag Algebra Proof of Theorem 1.11 for $(p_1, p_2) = (1/3, 2/3)$

We verify the inequality in Lemma 5.8 with $(p_1, p_2) = (1/3, 2/3)$ and $(H_1, H_2) = (C_4, C_5)$ for each graph $J$ on 5 vertices. There are 34 such graphs, labelled $J_1$ to $J_{34}$.

$J_1$ : 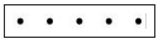

$$\frac{t_{\text{inj}}(C_4, J_1)}{4(1/3)^3} + \frac{t_{\text{inj}}(C_5, \overline{J_1})}{5(2/3)^4} - \frac{120}{120} \cdot A_1(1,1)$$

$$= \frac{0}{120 \cdot 4(1/3)^3} + \frac{120}{120 \cdot 5(2/3)^4} - \frac{120}{120} \cdot \frac{42246144}{53084160}$$

$$= \frac{13}{60}.$$

$J_2$ : 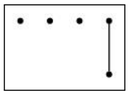

$$\frac{t_{\text{inj}}(C_4, J_2)}{4(1/3)^3} + \frac{t_{\text{inj}}(C_5, \overline{J_2})}{5(2/3)^4} - \frac{12}{120} \cdot A_1(1,1) - \frac{12}{120} \cdot A_1(1,2) - \frac{12}{120} \cdot A_1(1,3) - \frac{12}{120} \cdot A_1(1,4)$$

$$- \frac{12}{120} \cdot A_1(2,1) - \frac{12}{120} \cdot A_1(3,1) - \frac{12}{120} \cdot A_1(4,1) - \frac{12}{120} \cdot A_2(1,1)$$

$$= \frac{0}{120 \cdot 4(1/3)^3} + \frac{60}{120 \cdot 5(2/3)^4} - \frac{12}{120} \cdot \frac{42246144}{53084160} - \frac{12}{120} \cdot \frac{582094}{53084160} - \frac{12}{120} \cdot \frac{582094}{53084160} - \frac{12}{120} \cdot \frac{582094}{53084160}$$

$$- \frac{12}{120} \cdot \frac{582094}{53084160} - \frac{12}{120} \cdot \frac{582094}{53084160} - \frac{12}{120} \cdot \frac{582094}{53084160} - \frac{12}{120} \cdot \frac{107984172}{53084160}$$

$$= \frac{13}{60}.$$

$J_3$ : 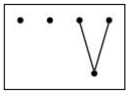

$$\frac{t_{\text{inj}}(C_4, J_3)}{4(1/3)^3} + \frac{t_{\text{inj}}(C_5, \overline{J_3})}{5(2/3)^4} - \frac{4}{120} \cdot A_1(1,2) - \frac{4}{120} \cdot A_1(1,3) - \frac{4}{120} \cdot A_1(1,4) - \frac{4}{120} \cdot A_1(1,5)$$

$$- \frac{4}{120} \cdot A_1(1,6) - \frac{4}{120} \cdot A_1(1,7) - \frac{4}{120} \cdot A_1(2,1) - \frac{4}{120} \cdot A_1(2,2) - \frac{4}{120} \cdot A_1(3,1) - \frac{4}{120} \cdot A_1(3,3)$$

$$-\frac{4}{120}\cdot A_1(4,1)-\frac{4}{120}\cdot A_1(4,4)-\frac{4}{120}\cdot A_1(5,1)-\frac{4}{120}\cdot A_1(6,1)-\frac{4}{120}\cdot A_1(7,1)-\frac{4}{120}\cdot A_2(1,2)$$
$$-\frac{4}{120}\cdot A_2(1,3)-\frac{4}{120}\cdot A_2(2,1)-\frac{4}{120}\cdot A_2(3,1)-\frac{4}{120}\cdot A_3(1,1)$$
$$=\frac{0}{120\cdot 4(1/3)^3}+\frac{20}{120\cdot 5(2/3)^4}-\frac{4}{120}\cdot\frac{582094}{53084160}-\frac{4}{120}\cdot\frac{582094}{53084160}-\frac{4}{120}\cdot\frac{582094}{53084160}+\frac{4}{120}\cdot\frac{42135552}{53084160}$$
$$+\frac{4}{120}\cdot\frac{42135552}{53084160}+\frac{4}{120}\cdot\frac{42135552}{53084160}-\frac{4}{120}\cdot\frac{582094}{53084160}-\frac{4}{120}\cdot\frac{49243392}{53084160}-\frac{4}{120}\cdot\frac{582094}{53084160}-\frac{4}{120}\cdot\frac{49243392}{53084160}$$
$$-\frac{4}{120}\cdot\frac{582094}{53084160}-\frac{4}{120}\cdot\frac{49243392}{53084160}+\frac{4}{120}\cdot\frac{42135552}{53084160}+\frac{4}{120}\cdot\frac{42135552}{53084160}+\frac{4}{120}\cdot\frac{42135552}{53084160}+\frac{4}{120}\cdot\frac{18972513}{53084160}$$
$$+\frac{4}{120}\cdot\frac{18972513}{53084160}+\frac{4}{120}\cdot\frac{18972513}{53084160}+\frac{4}{120}\cdot\frac{18972513}{53084160}-\frac{4}{120}\cdot\frac{101172144}{53084160}$$
$$=\frac{13}{60}.$$

$J_4$ : 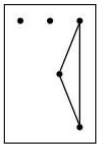

$$\frac{t_{\mathrm{inj}}(C_4,J_4)}{4(1/3)^3}+\frac{t_{\mathrm{inj}}(C_5,\overline{J_4})}{5(2/3)^4}-\frac{12}{120}\cdot A_1(2,2)-\frac{12}{120}\cdot A_1(3,3)-\frac{12}{120}\cdot A_1(4,4)-\frac{12}{120}\cdot A_2(1,5)$$
$$-\frac{12}{120}\cdot A_2(5,1)-\frac{12}{120}\cdot A_4(1,1)$$
$$=\frac{0}{120\cdot 4(1/3)^3}+\frac{0}{120\cdot 5(2/3)^4}-\frac{12}{120}\cdot\frac{49243392}{53084160}-\frac{12}{120}\cdot\frac{49243392}{53084160}-\frac{12}{120}\cdot\frac{49243392}{53084160}+\frac{12}{120}\cdot\frac{163858752}{53084160}$$
$$+\frac{12}{120}\cdot\frac{163858752}{53084160}-\frac{12}{120}\cdot\frac{64971648}{53084160}$$
$$=\frac{13}{60}.$$

$J_5$ : 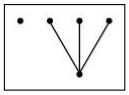

$$\frac{t_{\mathrm{inj}}(C_4,J_5)}{4(1/3)^3}+\frac{t_{\mathrm{inj}}(C_5,\overline{J_5})}{5(2/3)^4}-\frac{6}{120}\cdot A_1(1,5)-\frac{6}{120}\cdot A_1(1,6)-\frac{6}{120}\cdot A_1(1,7)-\frac{6}{120}\cdot A_1(1,8)$$
$$-\frac{6}{120}\cdot A_1(5,1)-\frac{6}{120}\cdot A_1(6,1)-\frac{6}{120}\cdot A_1(7,1)-\frac{6}{120}\cdot A_1(8,1)-\frac{6}{120}\cdot A_2(2,2)-\frac{6}{120}\cdot A_2(3,3)$$
$$-\frac{6}{120}\cdot A_3(1,2)-\frac{6}{120}\cdot A_3(2,1)$$

$$= \frac{0}{120 \cdot 4(1/3)^3} + \frac{0}{120 \cdot 5(2/3)^4} + \frac{6}{120} \cdot \frac{42135552}{53084160} + \frac{6}{120} \cdot \frac{42135552}{53084160} + \frac{6}{120} \cdot \frac{42135552}{53084160} + \frac{6}{120} \cdot \frac{92141034}{53084160}$$
$$+ \frac{6}{120} \cdot \frac{42135552}{53084160} + \frac{6}{120} \cdot \frac{42135552}{53084160} + \frac{6}{120} \cdot \frac{42135552}{53084160} + \frac{6}{120} \cdot \frac{92141034}{53084160} - \frac{6}{120} \cdot \frac{98249718}{53084160} - \frac{6}{120} \cdot \frac{98249718}{53084160}$$
$$- \frac{6}{120} \cdot \frac{5282292}{53084160} - \frac{6}{120} \cdot \frac{5282292}{53084160}$$
$$= \frac{13}{60}.$$

$J_6$ : 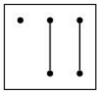

$$\frac{t_{\text{inj}}(C_4, J_6)}{4(1/3)^3} + \frac{t_{\text{inj}}(C_5, \overline{J_6})}{5(2/3)^4} - \frac{8}{120} \cdot A_1(2,3) - \frac{8}{120} \cdot A_1(2,4) - \frac{8}{120} \cdot A_1(3,2) - \frac{8}{120} \cdot A_1(3,4)$$
$$- \frac{8}{120} \cdot A_1(4,2) - \frac{8}{120} \cdot A_1(4,3) - \frac{8}{120} \cdot A_2(1,1) - \frac{8}{120} \cdot A_2(1,4) - \frac{8}{120} \cdot A_2(4,1)$$
$$= \frac{0}{120 \cdot 4(1/3)^3} + \frac{40}{120 \cdot 5(2/3)^4} + \frac{8}{120} \cdot \frac{15842304}{53084160} + \frac{8}{120} \cdot \frac{15842304}{53084160} + \frac{8}{120} \cdot \frac{15842304}{53084160} + \frac{8}{120} \cdot \frac{15842304}{53084160}$$
$$+ \frac{8}{120} \cdot \frac{15842304}{53084160} + \frac{8}{120} \cdot \frac{15842304}{53084160} - \frac{8}{120} \cdot \frac{107984172}{53084160} - \frac{8}{120} \cdot \frac{41642346}{53084160} - \frac{8}{120} \cdot \frac{41642346}{53084160}$$
$$= \frac{13}{60}.$$

$J_7$ : 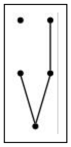

$$\frac{t_{\text{inj}}(C_4, J_7)}{4(1/3)^3} + \frac{t_{\text{inj}}(C_5, \overline{J_7})}{5(2/3)^4} - \frac{2}{120} \cdot A_1(2,3) - \frac{2}{120} \cdot A_1(2,4) - \frac{2}{120} \cdot A_1(2,5) - \frac{2}{120} \cdot A_1(2,6)$$
$$- \frac{2}{120} \cdot A_1(3,2) - \frac{2}{120} \cdot A_1(3,4) - \frac{2}{120} \cdot A_1(3,5) - \frac{2}{120} \cdot A_1(3,7) - \frac{2}{120} \cdot A_1(4,2) - \frac{2}{120} \cdot A_1(4,3)$$
$$- \frac{2}{120} \cdot A_1(4,6) - \frac{2}{120} \cdot A_1(4,7) - \frac{2}{120} \cdot A_1(5,2) - \frac{2}{120} \cdot A_1(5,3) - \frac{2}{120} \cdot A_1(6,2) - \frac{2}{120} \cdot A_1(6,4)$$
$$- \frac{2}{120} \cdot A_1(7,3) - \frac{2}{120} \cdot A_1(7,4) - \frac{2}{120} \cdot A_2(1,2) - \frac{2}{120} \cdot A_2(1,3) - \frac{2}{120} \cdot A_2(1,6) - \frac{2}{120} \cdot A_2(1,7)$$
$$- \frac{2}{120} \cdot A_2(2,1) - \frac{2}{120} \cdot A_2(2,3) - \frac{2}{120} \cdot A_2(3,1) - \frac{2}{120} \cdot A_2(3,2) - \frac{2}{120} \cdot A_2(6,1) - \frac{2}{120} \cdot A_2(7,1)$$
$$- \frac{2}{120} \cdot A_3(1,3) - \frac{2}{120} \cdot A_3(1,4) - \frac{2}{120} \cdot A_3(3,1) - \frac{2}{120} \cdot A_3(4,1)$$

$$= \frac{0}{120\cdot 4(1/3)^3} + \frac{10}{120\cdot 5(2/3)^4} + \frac{2}{120}\cdot\frac{15842304}{53084160} + \frac{2}{120}\cdot\frac{15842304}{53084160} - \frac{2}{120}\cdot\frac{7796736}{53084160} - \frac{2}{120}\cdot\frac{7796736}{53084160}$$
$$+\frac{2}{120}\cdot\frac{15842304}{53084160} + \frac{2}{120}\cdot\frac{15842304}{53084160} - \frac{2}{120}\cdot\frac{7796736}{53084160} - \frac{2}{120}\cdot\frac{7796736}{53084160} + \frac{2}{120}\cdot\frac{15842304}{53084160} + \frac{2}{120}\cdot\frac{15842304}{53084160}$$
$$-\frac{2}{120}\cdot\frac{7796736}{53084160} - \frac{2}{120}\cdot\frac{7796736}{53084160} - \frac{2}{120}\cdot\frac{7796736}{53084160} - \frac{2}{120}\cdot\frac{7796736}{53084160} - \frac{2}{120}\cdot\frac{7796736}{53084160} - \frac{2}{120}\cdot\frac{7796736}{53084160}$$
$$-\frac{2}{120}\cdot\frac{7796736}{53084160} - \frac{2}{120}\cdot\frac{7796736}{53084160} + \frac{2}{120}\cdot\frac{18972513}{53084160} + \frac{2}{120}\cdot\frac{18972513}{53084160} + \frac{2}{120}\cdot\frac{76966047}{53084160} + \frac{2}{120}\cdot\frac{76966047}{53084160}$$
$$+\frac{2}{120}\cdot\frac{18972513}{53084160} + \frac{2}{120}\cdot\frac{4893696}{53084160} + \frac{2}{120}\cdot\frac{18972513}{53084160} + \frac{2}{120}\cdot\frac{4893696}{53084160} + \frac{2}{120}\cdot\frac{76966047}{53084160} + \frac{2}{120}\cdot\frac{76966047}{53084160}$$
$$+\frac{2}{120}\cdot\frac{6580224}{53084160} + \frac{2}{120}\cdot\frac{6580224}{53084160} + \frac{2}{120}\cdot\frac{6580224}{53084160} + \frac{2}{120}\cdot\frac{6580224}{53084160}$$
$$= \frac{13}{60}.$$

$J_8$ : 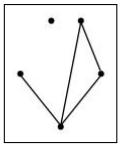

$$\frac{t_{\text{inj}}(C_4, J_8)}{4(1/3)^3} + \frac{t_{\text{inj}}(C_5, \overline{J_8})}{5(2/3)^4} - \frac{2}{120}\cdot A_1(2,5) - \frac{2}{120}\cdot A_1(2,6) - \frac{2}{120}\cdot A_1(3,5) - \frac{2}{120}\cdot A_1(3,7)$$
$$-\frac{2}{120}\cdot A_1(4,6) - \frac{2}{120}\cdot A_1(4,7) - \frac{2}{120}\cdot A_1(5,2) - \frac{2}{120}\cdot A_1(5,3) - \frac{2}{120}\cdot A_1(6,2) - \frac{2}{120}\cdot A_1(6,4)$$
$$-\frac{2}{120}\cdot A_1(7,3) - \frac{2}{120}\cdot A_1(7,4) - \frac{2}{120}\cdot A_2(1,5) - \frac{2}{120}\cdot A_2(1,8) - \frac{2}{120}\cdot A_2(2,2) - \frac{2}{120}\cdot A_2(2,5)$$
$$-\frac{2}{120}\cdot A_2(3,3) - \frac{2}{120}\cdot A_2(3,5) - \frac{2}{120}\cdot A_2(5,1) - \frac{2}{120}\cdot A_2(5,2) - \frac{2}{120}\cdot A_2(5,3) - \frac{2}{120}\cdot A_2(8,1)$$
$$-\frac{2}{120}\cdot A_3(1,5) - \frac{2}{120}\cdot A_3(1,6) - \frac{2}{120}\cdot A_3(5,1) - \frac{2}{120}\cdot A_3(6,1) - \frac{2}{120}\cdot A_4(1,2) - \frac{2}{120}\cdot A_4(1,3)$$
$$-\frac{2}{120}\cdot A_4(1,4) - \frac{2}{120}\cdot A_4(2,1) - \frac{2}{120}\cdot A_4(3,1) - \frac{2}{120}\cdot A_4(4,1)$$
$$= \frac{0}{120\cdot 4(1/3)^3} + \frac{0}{120\cdot 5(2/3)^4} - \frac{2}{120}\cdot\frac{7796736}{53084160} - \frac{2}{120}\cdot\frac{7796736}{53084160} - \frac{2}{120}\cdot\frac{7796736}{53084160} - \frac{2}{120}\cdot\frac{7796736}{53084160}$$
$$-\frac{2}{120}\cdot\frac{7796736}{53084160} - \frac{2}{120}\cdot\frac{7796736}{53084160} - \frac{2}{120}\cdot\frac{7796736}{53084160} - \frac{2}{120}\cdot\frac{7796736}{53084160} - \frac{2}{120}\cdot\frac{7796736}{53084160} - \frac{2}{120}\cdot\frac{7796736}{53084160}$$
$$-\frac{2}{120}\cdot\frac{7796736}{53084160} - \frac{2}{120}\cdot\frac{7796736}{53084160} + \frac{2}{120}\cdot\frac{163858752}{53084160} + \frac{2}{120}\cdot\frac{243081216}{53084160} - \frac{2}{120}\cdot\frac{98249718}{53084160} - \frac{2}{120}\cdot\frac{56408379}{53084160}$$
$$-\frac{2}{120}\cdot\frac{98249718}{53084160} - \frac{2}{120}\cdot\frac{56408379}{53084160} + \frac{2}{120}\cdot\frac{163858752}{53084160} - \frac{2}{120}\cdot\frac{56408379}{53084160} - \frac{2}{120}\cdot\frac{56408379}{53084160} + \frac{2}{120}\cdot\frac{243081216}{53084160}$$

$$+\frac{2}{120}\cdot\frac{85681152}{53084160}+\frac{2}{120}\cdot\frac{85681152}{53084160}+\frac{2}{120}\cdot\frac{85681152}{53084160}+\frac{2}{120}\cdot\frac{85681152}{53084160}+\frac{2}{120}\cdot\frac{8197220}{53084160}+\frac{2}{120}\cdot\frac{8197220}{53084160}$$

$$+\frac{2}{120}\cdot\frac{8197220}{53084160}+\frac{2}{120}\cdot\frac{8197220}{53084160}+\frac{2}{120}\cdot\frac{8197220}{53084160}+\frac{2}{120}\cdot\frac{8197220}{53084160}$$

$$=\frac{13}{60}.$$

$J_9$ : 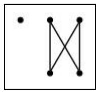

$$\frac{t_{\text{inj}}(C_4,J_9)}{4(1/3)^3}+\frac{t_{\text{inj}}(C_5,\overline{J_9})}{5(2/3)^4}-\frac{8}{120}\cdot A_1(5,5)-\frac{8}{120}\cdot A_1(6,6)-\frac{8}{120}\cdot A_1(7,7)-\frac{8}{120}\cdot A_2(2,3)$$

$$-\frac{8}{120}\cdot A_2(3,2)-\frac{8}{120}\cdot A_3(1,7)-\frac{8}{120}\cdot A_3(7,1)$$

$$=\frac{8}{120\cdot 4(1/3)^3}+\frac{0}{120\cdot 5(2/3)^4}-\frac{8}{120}\cdot\frac{138599424}{53084160}-\frac{8}{120}\cdot\frac{138599424}{53084160}-\frac{8}{120}\cdot\frac{138599424}{53084160}+\frac{8}{120}\cdot\frac{4893696}{53084160}$$

$$+\frac{8}{120}\cdot\frac{4893696}{53084160}+\frac{8}{120}\cdot\frac{110108160}{53084160}+\frac{8}{120}\cdot\frac{110108160}{53084160}$$

$$=\frac{13}{60}.$$

$J_{10}$ : 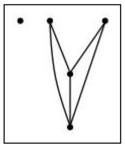

$$\frac{t_{\text{inj}}(C_4,J_{10})}{4(1/3)^3}+\frac{t_{\text{inj}}(C_5,\overline{J_{10}})}{5(2/3)^4}-\frac{4}{120}\cdot A_1(5,5)-\frac{4}{120}\cdot A_1(6,6)-\frac{4}{120}\cdot A_1(7,7)-\frac{4}{120}\cdot A_2(2,5)$$

$$-\frac{4}{120}\cdot A_2(3,5)-\frac{4}{120}\cdot A_2(5,2)-\frac{4}{120}\cdot A_2(5,3)-\frac{4}{120}\cdot A_2(5,5)-\frac{4}{120}\cdot A_3(1,8)-\frac{4}{120}\cdot A_3(8,1)$$

$$-\frac{4}{120}\cdot A_4(1,5)-\frac{4}{120}\cdot A_4(1,6)-\frac{4}{120}\cdot A_4(1,7)-\frac{4}{120}\cdot A_4(5,1)-\frac{4}{120}\cdot A_4(6,1)-\frac{4}{120}\cdot A_4(7,1)$$

$$=\frac{8}{120\cdot 4(1/3)^3}+\frac{0}{120\cdot 5(2/3)^4}-\frac{4}{120}\cdot\frac{138599424}{53084160}-\frac{4}{120}\cdot\frac{138599424}{53084160}-\frac{4}{120}\cdot\frac{138599424}{53084160}-\frac{4}{120}\cdot\frac{56408379}{53084160}$$

$$-\frac{4}{120}\cdot\frac{56408379}{53084160}-\frac{4}{120}\cdot\frac{56408379}{53084160}-\frac{4}{120}\cdot\frac{56408379}{53084160}-\frac{4}{120}\cdot\frac{487876608}{53084160}+\frac{4}{120}\cdot\frac{214922952}{53084160}+\frac{4}{120}\cdot\frac{214922952}{53084160}$$

$$+\frac{4}{120}\cdot\frac{54645562}{53084160}+\frac{4}{120}\cdot\frac{54645562}{53084160}+\frac{4}{120}\cdot\frac{54645562}{53084160}+\frac{4}{120}\cdot\frac{54645562}{53084160}+\frac{4}{120}\cdot\frac{54645562}{53084160}+\frac{4}{120}\cdot\frac{54645562}{53084160}$$

$$= \frac{13}{60}.$$

$J_{11}$ : 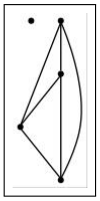

$$\frac{t_{\text{inj}}(C_4, J_{11})}{4(1/3)^3} + \frac{t_{\text{inj}}(C_5, \overline{J_{11}})}{5(2/3)^4} - \frac{24}{120} \cdot A_2(5,5) - \frac{24}{120} \cdot A_4(1,8) - \frac{24}{120} \cdot A_4(8,1)$$

$$= \frac{24}{120 \cdot 4(1/3)^3} + \frac{0}{120 \cdot 5(2/3)^4} - \frac{24}{120} \cdot \frac{487876608}{53084160} + \frac{24}{120} \cdot \frac{93533184}{53084160} + \frac{24}{120} \cdot \frac{93533184}{53084160}$$

$$= \frac{13}{60}.$$

$J_{12}$ : 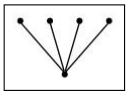

$$\frac{t_{\text{inj}}(C_4, J_{12})}{4(1/3)^3} + \frac{t_{\text{inj}}(C_5, \overline{J_{12}})}{5(2/3)^4} - \frac{24}{120} \cdot A_1(1,8) - \frac{24}{120} \cdot A_1(8,1) - \frac{24}{120} \cdot A_3(2,2)$$

$$= \frac{0}{120 \cdot 4(1/3)^3} + \frac{0}{120 \cdot 5(2/3)^4} + \frac{24}{120} \cdot \frac{92141034}{53084160} + \frac{24}{120} \cdot \frac{92141034}{53084160} - \frac{24}{120} \cdot \frac{126774228}{53084160}$$

$$= \frac{13}{60}.$$

$J_{13}$ : 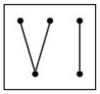

$$\frac{t_{\text{inj}}(C_4, J_{13})}{4(1/3)^3} + \frac{t_{\text{inj}}(C_5, \overline{J_{13}})}{5(2/3)^4} - \frac{4}{120} \cdot A_1(2,7) - \frac{4}{120} \cdot A_1(3,6) - \frac{4}{120} \cdot A_1(4,5) - \frac{4}{120} \cdot A_1(5,4)$$

$$- \frac{4}{120} \cdot A_1(6,3) - \frac{4}{120} \cdot A_1(7,2) - \frac{4}{120} \cdot A_2(1,4) - \frac{4}{120} \cdot A_2(2,4) - \frac{4}{120} \cdot A_2(3,4) - \frac{4}{120} \cdot A_2(4,1)$$

$$- \frac{4}{120} \cdot A_2(4,2) - \frac{4}{120} \cdot A_2(4,3) - \frac{4}{120} \cdot A_2(4,4) - \frac{4}{120} \cdot A_3(1,1)$$

$$= \frac{0}{120 \cdot 4(1/3)^3} + \frac{20}{120 \cdot 5(2/3)^4} + \frac{4}{120} \cdot \frac{46514496}{53084160} + \frac{4}{120} \cdot \frac{46514496}{53084160} + \frac{4}{120} \cdot \frac{46514496}{53084160} + \frac{4}{120} \cdot \frac{46514496}{53084160}$$

$$+ \frac{4}{120} \cdot \frac{46514496}{53084160} + \frac{4}{120} \cdot \frac{46514496}{53084160} - \frac{4}{120} \cdot \frac{41642346}{53084160} + \frac{4}{120} \cdot \frac{36052992}{53084160} + \frac{4}{120} \cdot \frac{36052992}{53084160} - \frac{4}{120} \cdot \frac{41642346}{53084160}$$

$$+\frac{4}{120}\cdot\frac{36052992}{53084160}+\frac{4}{120}\cdot\frac{36052992}{53084160}-\frac{4}{120}\cdot\frac{162533628}{53084160}-\frac{4}{120}\cdot\frac{101172144}{53084160}$$
$$=\frac{13}{60}.$$

$J_{14}$ : 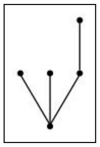

$$\frac{t_{\mathrm{inj}}(C_4,J_{14})}{4(1/3)^3}+\frac{t_{\mathrm{inj}}(C_5,\overline{J_{14}})}{5(2/3)^4}-\frac{2}{120}\cdot A_1(2,7)-\frac{2}{120}\cdot A_1(2,8)-\frac{2}{120}\cdot A_1(3,6)-\frac{2}{120}\cdot A_1(3,8)$$
$$-\frac{2}{120}\cdot A_1(4,5)-\frac{2}{120}\cdot A_1(4,8)-\frac{2}{120}\cdot A_1(5,4)-\frac{2}{120}\cdot A_1(6,3)-\frac{2}{120}\cdot A_1(7,2)-\frac{2}{120}\cdot A_1(8,2)$$
$$-\frac{2}{120}\cdot A_1(8,3)-\frac{2}{120}\cdot A_1(8,4)-\frac{2}{120}\cdot A_2(1,6)-\frac{2}{120}\cdot A_2(1,7)-\frac{2}{120}\cdot A_2(2,6)-\frac{2}{120}\cdot A_2(3,7)$$
$$-\frac{2}{120}\cdot A_2(6,1)-\frac{2}{120}\cdot A_2(6,2)-\frac{2}{120}\cdot A_2(7,1)-\frac{2}{120}\cdot A_2(7,3)-\frac{2}{120}\cdot A_3(1,2)-\frac{2}{120}\cdot A_3(2,1)$$
$$-\frac{2}{120}\cdot A_3(2,3)-\frac{2}{120}\cdot A_3(2,4)-\frac{2}{120}\cdot A_3(3,2)-\frac{2}{120}\cdot A_3(3,3)-\frac{2}{120}\cdot A_3(4,2)-\frac{2}{120}\cdot A_3(4,4)$$

$$=\frac{0}{120\cdot 4(1/3)^3}+\frac{0}{120\cdot 5(2/3)^4}+\frac{2}{120}\cdot\frac{46514496}{53084160}+\frac{2}{120}\cdot\frac{13049856}{53084160}+\frac{2}{120}\cdot\frac{46514496}{53084160}+\frac{2}{120}\cdot\frac{13049856}{53084160}$$
$$+\frac{2}{120}\cdot\frac{46514496}{53084160}+\frac{2}{120}\cdot\frac{13049856}{53084160}+\frac{2}{120}\cdot\frac{46514496}{53084160}+\frac{2}{120}\cdot\frac{46514496}{53084160}+\frac{2}{120}\cdot\frac{46514496}{53084160}+\frac{2}{120}\cdot\frac{13049856}{53084160}$$
$$+\frac{2}{120}\cdot\frac{13049856}{53084160}+\frac{2}{120}\cdot\frac{13049856}{53084160}+\frac{2}{120}\cdot\frac{76966047}{53084160}+\frac{2}{120}\cdot\frac{76966047}{53084160}+\frac{2}{120}\cdot\frac{75589632}{53084160}+\frac{2}{120}\cdot\frac{75589632}{53084160}$$
$$+\frac{2}{120}\cdot\frac{76966047}{53084160}+\frac{2}{120}\cdot\frac{75589632}{53084160}+\frac{2}{120}\cdot\frac{76966047}{53084160}+\frac{2}{120}\cdot\frac{75589632}{53084160}-\frac{2}{120}\cdot\frac{5282292}{53084160}-\frac{2}{120}\cdot\frac{5282292}{53084160}$$
$$+\frac{2}{120}\cdot\frac{8879739}{53084160}+\frac{2}{120}\cdot\frac{8879739}{53084160}+\frac{2}{120}\cdot\frac{8879739}{53084160}-\frac{2}{120}\cdot\frac{151234560}{53084160}+\frac{2}{120}\cdot\frac{8879739}{53084160}-\frac{2}{120}\cdot\frac{151234560}{53084160}$$

$$=\frac{13}{60}.$$

$J_{15}$ : 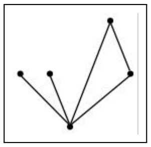

$$\frac{t_{\mathrm{inj}}(C_4,J_{15})}{4(1/3)^3}+\frac{t_{\mathrm{inj}}(C_5,\overline{J_{15}})}{5(2/3)^4}-\frac{4}{120}\cdot A_1(2,8)-\frac{4}{120}\cdot A_1(3,8)-\frac{4}{120}\cdot A_1(4,8)-\frac{4}{120}\cdot A_1(8,2)$$

$$-\frac{4}{120}\cdot A_1(8,3)-\frac{4}{120}\cdot A_1(8,4)-\frac{4}{120}\cdot A_2(1,8)-\frac{4}{120}\cdot A_2(8,1)-\frac{4}{120}\cdot A_3(2,2)-\frac{4}{120}\cdot A_3(2,5)$$
$$-\frac{4}{120}\cdot A_3(2,6)-\frac{4}{120}\cdot A_3(5,2)-\frac{4}{120}\cdot A_3(6,2)-\frac{4}{120}\cdot A_4(2,2)-\frac{4}{120}\cdot A_4(3,3)-\frac{4}{120}\cdot A_4(4,4)$$

$$=\frac{0}{120\cdot 4(1/3)^3}+\frac{0}{120\cdot 5(2/3)^4}+\frac{4}{120}\cdot\frac{13049856}{53084160}+\frac{4}{120}\cdot\frac{13049856}{53084160}+\frac{4}{120}\cdot\frac{13049856}{53084160}+\frac{4}{120}\cdot\frac{13049856}{53084160}$$
$$+\frac{4}{120}\cdot\frac{13049856}{53084160}+\frac{4}{120}\cdot\frac{13049856}{53084160}+\frac{4}{120}\cdot\frac{243081216}{53084160}+\frac{4}{120}\cdot\frac{243081216}{53084160}-\frac{4}{120}\cdot\frac{126774228}{53084160}+\frac{4}{120}\cdot\frac{55406592}{53084160}$$
$$+\frac{4}{120}\cdot\frac{55406592}{53084160}+\frac{4}{120}\cdot\frac{55406592}{53084160}+\frac{4}{120}\cdot\frac{55406592}{53084160}-\frac{4}{120}\cdot\frac{104755556}{53084160}-\frac{4}{120}\cdot\frac{104755556}{53084160}-\frac{4}{120}\cdot\frac{104755556}{53084160}$$

$$=\frac{13}{60}.$$

$J_{16}$ : 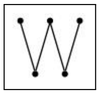

$$\frac{t_{\mathrm{inj}}(C_4,J_{16})}{4(1/3)^3}+\frac{t_{\mathrm{inj}}(C_5,\overline{J_{16}})}{5(2/3)^4}-\frac{2}{120}\cdot A_1(5,6)-\frac{2}{120}\cdot A_1(5,7)-\frac{2}{120}\cdot A_1(6,5)-\frac{2}{120}\cdot A_1(6,7)$$

$$-\frac{2}{120}\cdot A_1(7,5)-\frac{2}{120}\cdot A_1(7,6)-\frac{2}{120}\cdot A_2(2,4)-\frac{2}{120}\cdot A_2(2,7)-\frac{2}{120}\cdot A_2(3,4)-\frac{2}{120}\cdot A_2(3,6)$$
$$-\frac{2}{120}\cdot A_2(4,2)-\frac{2}{120}\cdot A_2(4,3)-\frac{2}{120}\cdot A_2(4,6)-\frac{2}{120}\cdot A_2(4,7)-\frac{2}{120}\cdot A_2(6,3)-\frac{2}{120}\cdot A_2(6,4)$$
$$-\frac{2}{120}\cdot A_2(7,2)-\frac{2}{120}\cdot A_2(7,4)-\frac{2}{120}\cdot A_3(1,3)-\frac{2}{120}\cdot A_3(1,4)-\frac{2}{120}\cdot A_3(3,1)-\frac{2}{120}\cdot A_3(3,4)$$
$$-\frac{2}{120}\cdot A_3(4,1)-\frac{2}{120}\cdot A_3(4,3)$$
$$=\frac{0}{120\cdot 4(1/3)^3}+\frac{10}{120\cdot 5(2/3)^4}-\frac{2}{120}\cdot\frac{21676032}{53084160}-\frac{2}{120}\cdot\frac{21676032}{53084160}-\frac{2}{120}\cdot\frac{21676032}{53084160}-\frac{2}{120}\cdot\frac{21676032}{53084160}$$
$$-\frac{2}{120}\cdot\frac{21676032}{53084160}-\frac{2}{120}\cdot\frac{21676032}{53084160}+\frac{2}{120}\cdot\frac{36052992}{53084160}+\frac{2}{120}\cdot\frac{25408512}{53084160}+\frac{2}{120}\cdot\frac{36052992}{53084160}+\frac{2}{120}\cdot\frac{25408512}{53084160}$$
$$+\frac{2}{120}\cdot\frac{36052992}{53084160}+\frac{2}{120}\cdot\frac{36052992}{53084160}+\frac{2}{120}\cdot\frac{38375424}{53084160}+\frac{2}{120}\cdot\frac{38375424}{53084160}+\frac{2}{120}\cdot\frac{25408512}{53084160}+\frac{2}{120}\cdot\frac{38375424}{53084160}$$
$$+\frac{2}{120}\cdot\frac{25408512}{53084160}+\frac{2}{120}\cdot\frac{38375424}{53084160}+\frac{2}{120}\cdot\frac{6580224}{53084160}+\frac{2}{120}\cdot\frac{6580224}{53084160}+\frac{2}{120}\cdot\frac{6580224}{53084160}+\frac{2}{120}\cdot\frac{62871552}{53084160}$$
$$+\frac{2}{120}\cdot\frac{6580224}{53084160}+\frac{2}{120}\cdot\frac{62871552}{53084160}$$
$$=\frac{13}{60}.$$

$J_{17}$ : 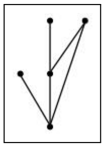

$$\frac{t_{\text{inj}}(C_4, J_{17})}{4(1/3)^3} + \frac{t_{\text{inj}}(C_5, \overline{J_{17}})}{5(2/3)^4} - \frac{2}{120}\cdot A_1(5,6) - \frac{2}{120}\cdot A_1(5,7) - \frac{2}{120}\cdot A_1(6,5) - \frac{2}{120}\cdot A_1(6,7)$$

$$-\frac{2}{120}\cdot A_1(7,5) - \frac{2}{120}\cdot A_1(7,6) - \frac{2}{120}\cdot A_2(2,6) - \frac{2}{120}\cdot A_2(2,8) - \frac{2}{120}\cdot A_2(3,7) - \frac{2}{120}\cdot A_2(3,8)$$
$$-\frac{2}{120}\cdot A_2(6,2) - \frac{2}{120}\cdot A_2(7,3) - \frac{2}{120}\cdot A_2(8,2) - \frac{2}{120}\cdot A_2(8,3) - \frac{2}{120}\cdot A_3(1,5) - \frac{2}{120}\cdot A_3(1,6)$$
$$-\frac{2}{120}\cdot A_3(3,5) - \frac{2}{120}\cdot A_3(4,6) - \frac{2}{120}\cdot A_3(5,1) - \frac{2}{120}\cdot A_3(5,3) - \frac{2}{120}\cdot A_3(6,1) - \frac{2}{120}\cdot A_3(6,4)$$
$$-\frac{2}{120}\cdot A_4(2,3) - \frac{2}{120}\cdot A_4(2,4) - \frac{2}{120}\cdot A_4(3,2) - \frac{2}{120}\cdot A_4(3,4) - \frac{2}{120}\cdot A_4(4,2) - \frac{2}{120}\cdot A_4(4,3)$$

$$= \frac{0}{120\cdot 4(1/3)^3} + \frac{0}{120\cdot 5(2/3)^4} - \frac{2}{120}\cdot\frac{21676032}{53084160} - \frac{2}{120}\cdot\frac{21676032}{53084160} - \frac{2}{120}\cdot\frac{21676032}{53084160} - \frac{2}{120}\cdot\frac{21676032}{53084160}$$
$$-\frac{2}{120}\cdot\frac{21676032}{53084160} - \frac{2}{120}\cdot\frac{21676032}{53084160} + \frac{2}{120}\cdot\frac{75589632}{53084160} - \frac{2}{120}\cdot\frac{11747760}{53084160} + \frac{2}{120}\cdot\frac{75589632}{53084160} - \frac{2}{120}\cdot\frac{11747760}{53084160}$$
$$+\frac{2}{120}\cdot\frac{75589632}{53084160} + \frac{2}{120}\cdot\frac{75589632}{53084160} - \frac{2}{120}\cdot\frac{11747760}{53084160} - \frac{2}{120}\cdot\frac{11747760}{53084160} + \frac{2}{120}\cdot\frac{85681152}{53084160} + \frac{2}{120}\cdot\frac{85681152}{53084160}$$
$$+\frac{2}{120}\cdot\frac{3815424}{53084160} + \frac{2}{120}\cdot\frac{3815424}{53084160} + \frac{2}{120}\cdot\frac{85681152}{53084160} + \frac{2}{120}\cdot\frac{3815424}{53084160} + \frac{2}{120}\cdot\frac{85681152}{53084160} + \frac{2}{120}\cdot\frac{3815424}{53084160}$$
$$+\frac{2}{120}\cdot\frac{34466080}{53084160} + \frac{2}{120}\cdot\frac{34466080}{53084160} + \frac{2}{120}\cdot\frac{34466080}{53084160} + \frac{2}{120}\cdot\frac{34466080}{53084160} + \frac{2}{120}\cdot\frac{34466080}{53084160} + \frac{2}{120}\cdot\frac{34466080}{53084160}$$

$$= \frac{13}{60}.$$

$J_{18}$ : 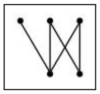

$$\frac{t_{\text{inj}}(C_4, J_{18})}{4(1/3)^3} + \frac{t_{\text{inj}}(C_5, \overline{J_{18}})}{5(2/3)^4} - \frac{2}{120}\cdot A_1(5,8) - \frac{2}{120}\cdot A_1(6,8) - \frac{2}{120}\cdot A_1(7,8) - \frac{2}{120}\cdot A_1(8,5)$$

$$-\frac{2}{120}\cdot A_1(8,6) - \frac{2}{120}\cdot A_1(8,7) - \frac{2}{120}\cdot A_2(2,7) - \frac{2}{120}\cdot A_2(3,6) - \frac{2}{120}\cdot A_2(6,3) - \frac{2}{120}\cdot A_2(6,6)$$
$$-\frac{2}{120}\cdot A_2(7,2) - \frac{2}{120}\cdot A_2(7,7) - \frac{2}{120}\cdot A_3(1,7) - \frac{2}{120}\cdot A_3(2,3) - \frac{2}{120}\cdot A_3(2,4) - \frac{2}{120}\cdot A_3(2,7)$$
$$-\frac{2}{120}\cdot A_3(3,2) - \frac{2}{120}\cdot A_3(3,7) - \frac{2}{120}\cdot A_3(4,2) - \frac{2}{120}\cdot A_3(4,7) - \frac{2}{120}\cdot A_3(7,1) - \frac{2}{120}\cdot A_3(7,2)$$

$$-\frac{2}{120}\cdot A_3(7,3)-\frac{2}{120}\cdot A_3(7,4)$$

$$= \frac{8}{120\cdot 4(1/3)^3}+\frac{0}{120\cdot 5(2/3)^4}-\frac{2}{120}\cdot\frac{96865624}{53084160}-\frac{2}{120}\cdot\frac{96865624}{53084160}-\frac{2}{120}\cdot\frac{96865624}{53084160}-\frac{2}{120}\cdot\frac{96865624}{53084160}$$

$$-\frac{2}{120}\cdot\frac{96865624}{53084160}-\frac{2}{120}\cdot\frac{96865624}{53084160}+\frac{2}{120}\cdot\frac{25408512}{53084160}+\frac{2}{120}\cdot\frac{25408512}{53084160}+\frac{2}{120}\cdot\frac{25408512}{53084160}-\frac{2}{120}\cdot\frac{359826702}{53084160}$$

$$+\frac{2}{120}\cdot\frac{25408512}{53084160}-\frac{2}{120}\cdot\frac{359826702}{53084160}+\frac{2}{120}\cdot\frac{110108160}{53084160}+\frac{2}{120}\cdot\frac{8879739}{53084160}+\frac{2}{120}\cdot\frac{8879739}{53084160}+\frac{2}{120}\cdot\frac{39429504}{53084160}$$

$$+\frac{2}{120}\cdot\frac{8879739}{53084160}+\frac{2}{120}\cdot\frac{30360144}{53084160}+\frac{2}{120}\cdot\frac{8879739}{53084160}+\frac{2}{120}\cdot\frac{30360144}{53084160}+\frac{2}{120}\cdot\frac{110108160}{53084160}+\frac{2}{120}\cdot\frac{39429504}{53084160}$$

$$+\frac{2}{120}\cdot\frac{30360144}{53084160}+\frac{2}{120}\cdot\frac{30360144}{53084160}$$

$$=\frac{13}{60}.$$

$J_{19}$ : 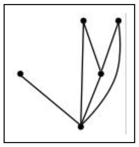

$$\frac{t_{\mathrm{inj}}(C_4,J_{19})}{4(1/3)^3}+\frac{t_{\mathrm{inj}}(C_5,\overline{J_{19}})}{5(2/3)^4}-\frac{2}{120}\cdot A_1(5,8)-\frac{2}{120}\cdot A_1(6,8)-\frac{2}{120}\cdot A_1(7,8)-\frac{2}{120}\cdot A_1(8,5)$$

$$-\frac{2}{120}\cdot A_1(8,6)-\frac{2}{120}\cdot A_1(8,7)-\frac{2}{120}\cdot A_2(2,8)-\frac{2}{120}\cdot A_2(3,8)-\frac{2}{120}\cdot A_2(8,2)-\frac{2}{120}\cdot A_2(8,3)$$

$$-\frac{2}{120}\cdot A_3(1,8)-\frac{2}{120}\cdot A_3(2,5)-\frac{2}{120}\cdot A_3(2,6)-\frac{2}{120}\cdot A_3(2,8)-\frac{2}{120}\cdot A_3(5,2)-\frac{2}{120}\cdot A_3(5,5)$$

$$-\frac{2}{120}\cdot A_3(6,2)-\frac{2}{120}\cdot A_3(6,6)-\frac{2}{120}\cdot A_3(8,1)-\frac{2}{120}\cdot A_3(8,2)-\frac{2}{120}\cdot A_4(2,5)-\frac{2}{120}\cdot A_4(2,6)$$

$$-\frac{2}{120}\cdot A_4(3,5)-\frac{2}{120}\cdot A_4(3,7)-\frac{2}{120}\cdot A_4(4,6)-\frac{2}{120}\cdot A_4(4,7)-\frac{2}{120}\cdot A_4(5,2)-\frac{2}{120}\cdot A_4(5,3)$$

$$-\frac{2}{120}\cdot A_4(6,2)-\frac{2}{120}\cdot A_4(6,4)-\frac{2}{120}\cdot A_4(7,3)-\frac{2}{120}\cdot A_4(7,4)$$

$$= \frac{8}{120\cdot 4(1/3)^3}+\frac{0}{120\cdot 5(2/3)^4}-\frac{2}{120}\cdot\frac{96865624}{53084160}-\frac{2}{120}\cdot\frac{96865624}{53084160}-\frac{2}{120}\cdot\frac{96865624}{53084160}-\frac{2}{120}\cdot\frac{96865624}{53084160}$$

$$-\frac{2}{120}\cdot\frac{96865624}{53084160}-\frac{2}{120}\cdot\frac{96865624}{53084160}-\frac{2}{120}\cdot\frac{11747760}{53084160}-\frac{2}{120}\cdot\frac{11747760}{53084160}-\frac{2}{120}\cdot\frac{11747760}{53084160}-\frac{2}{120}\cdot\frac{11747760}{53084160}$$

$$+\frac{2}{120}\cdot\frac{214922952}{53084160}+\frac{2}{120}\cdot\frac{55406592}{53084160}+\frac{2}{120}\cdot\frac{55406592}{53084160}+\frac{2}{120}\cdot\frac{177831936}{53084160}+\frac{2}{120}\cdot\frac{55406592}{53084160}-\frac{2}{120}\cdot\frac{466255872}{53084160}$$

$$+\frac{2}{120}\cdot\frac{55406592}{53084160}-\frac{2}{120}\cdot\frac{466255872}{53084160}+\frac{2}{120}\cdot\frac{214922952}{53084160}+\frac{2}{120}\cdot\frac{177831936}{53084160}-\frac{2}{120}\cdot\frac{15801488}{53084160}-\frac{2}{120}\cdot\frac{15801488}{53084160}$$

$$-\frac{2}{120}\cdot\frac{15801488}{53084160}-\frac{2}{120}\cdot\frac{15801488}{53084160}-\frac{2}{120}\cdot\frac{15801488}{53084160}-\frac{2}{120}\cdot\frac{15801488}{53084160}-\frac{2}{120}\cdot\frac{15801488}{53084160}-\frac{2}{120}\cdot\frac{15801488}{53084160}$$
$$-\frac{2}{120}\cdot\frac{15801488}{53084160}-\frac{2}{120}\cdot\frac{15801488}{53084160}-\frac{2}{120}\cdot\frac{15801488}{53084160}-\frac{2}{120}\cdot\frac{15801488}{53084160}$$
$$=\frac{13}{60}.$$

$J_{20}$ : 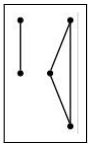

$$\frac{t_{\mathrm{inj}}(C_4,J_{20})}{4(1/3)^3}+\frac{t_{\mathrm{inj}}(C_5,\overline{J_{20}})}{5(2/3)^4}-\frac{12}{120}\cdot A_2(4,4)-\frac{12}{120}\cdot A_2(4,5)-\frac{12}{120}\cdot A_2(5,4)-\frac{12}{120}\cdot A_4(1,1)$$

$$=\frac{0}{120\cdot 4(1/3)^3}+\frac{0}{120\cdot 5(2/3)^4}-\frac{12}{120}\cdot\frac{162533628}{53084160}+\frac{12}{120}\cdot\frac{171260478}{53084160}+\frac{12}{120}\cdot\frac{171260478}{53084160}-\frac{12}{120}\cdot\frac{64971648}{53084160}$$

$$=\frac{13}{60}.$$

$J_{21}$ : 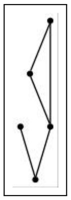

$$\frac{t_{\mathrm{inj}}(C_4,J_{21})}{4(1/3)^3}+\frac{t_{\mathrm{inj}}(C_5,\overline{J_{21}})}{5(2/3)^4}-\frac{2}{120}\cdot A_2(4,5)-\frac{2}{120}\cdot A_2(4,6)-\frac{2}{120}\cdot A_2(4,7)-\frac{2}{120}\cdot A_2(4,8)$$

$$-\frac{2}{120}\cdot A_2(5,4)-\frac{2}{120}\cdot A_2(5,6)-\frac{2}{120}\cdot A_2(5,7)-\frac{2}{120}\cdot A_2(6,4)-\frac{2}{120}\cdot A_2(6,5)-\frac{2}{120}\cdot A_2(7,4)$$
$$-\frac{2}{120}\cdot A_2(7,5)-\frac{2}{120}\cdot A_2(8,4)-\frac{2}{120}\cdot A_3(3,3)-\frac{2}{120}\cdot A_3(3,6)-\frac{2}{120}\cdot A_3(4,4)-\frac{2}{120}\cdot A_3(4,5)$$
$$-\frac{2}{120}\cdot A_3(5,4)-\frac{2}{120}\cdot A_3(6,3)-\frac{2}{120}\cdot A_4(1,2)-\frac{2}{120}\cdot A_4(1,3)-\frac{2}{120}\cdot A_4(1,4)-\frac{2}{120}\cdot A_4(2,1)$$
$$-\frac{2}{120}\cdot A_4(3,1)-\frac{2}{120}\cdot A_4(4,1)$$
$$=\frac{0}{120\cdot 4(1/3)^3}+\frac{0}{120\cdot 5(2/3)^4}+\frac{2}{120}\cdot\frac{171260478}{53084160}+\frac{2}{120}\cdot\frac{38375424}{53084160}+\frac{2}{120}\cdot\frac{38375424}{53084160}+\frac{2}{120}\cdot\frac{198826518}{53084160}$$
$$+\frac{2}{120}\cdot\frac{171260478}{53084160}-\frac{2}{120}\cdot\frac{83816640}{53084160}-\frac{2}{120}\cdot\frac{83816640}{53084160}+\frac{2}{120}\cdot\frac{38375424}{53084160}-\frac{2}{120}\cdot\frac{83816640}{53084160}+\frac{2}{120}\cdot\frac{38375424}{53084160}$$

$$-\frac{2}{120}\cdot\frac{83816640}{53084160}+\frac{2}{120}\cdot\frac{198826518}{53084160}-\frac{2}{120}\cdot\frac{151234560}{53084160}+\frac{2}{120}\cdot\frac{96242688}{53084160}-\frac{2}{120}\cdot\frac{151234560}{53084160}+\frac{2}{120}\cdot\frac{96242688}{53084160}$$
$$+\frac{2}{120}\cdot\frac{96242688}{53084160}+\frac{2}{120}\cdot\frac{96242688}{53084160}+\frac{2}{120}\cdot\frac{8197220}{53084160}+\frac{2}{120}\cdot\frac{8197220}{53084160}+\frac{2}{120}\cdot\frac{8197220}{53084160}+\frac{2}{120}\cdot\frac{8197220}{53084160}$$
$$+\frac{2}{120}\cdot\frac{8197220}{53084160}+\frac{2}{120}\cdot\frac{8197220}{53084160}$$
$$=\frac{13}{60}.$$

$J_{22}$ : 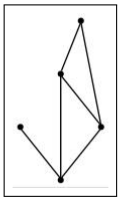

$$\frac{t_{\text{inj}}(C_4,J_{22})}{4(1/3)^3}+\frac{t_{\text{inj}}(C_5,\overline{J_{22}})}{5(2/3)^4}-\frac{2}{120}\cdot A_2(5,6)-\frac{2}{120}\cdot A_2(5,7)-\frac{2}{120}\cdot A_2(5,8)-\frac{2}{120}\cdot A_2(6,5)$$
$$-\frac{2}{120}\cdot A_2(6,6)-\frac{2}{120}\cdot A_2(7,5)-\frac{2}{120}\cdot A_2(7,7)-\frac{2}{120}\cdot A_2(8,5)-\frac{2}{120}\cdot A_3(3,5)-\frac{2}{120}\cdot A_3(3,8)$$
$$-\frac{2}{120}\cdot A_3(4,6)-\frac{2}{120}\cdot A_3(4,8)-\frac{2}{120}\cdot A_3(5,3)-\frac{2}{120}\cdot A_3(6,4)-\frac{2}{120}\cdot A_3(8,3)-\frac{2}{120}\cdot A_3(8,4)$$
$$-\frac{2}{120}\cdot A_4(1,5)-\frac{2}{120}\cdot A_4(1,6)-\frac{2}{120}\cdot A_4(1,7)-\frac{2}{120}\cdot A_4(2,7)-\frac{2}{120}\cdot A_4(3,6)-\frac{2}{120}\cdot A_4(4,5)$$
$$-\frac{2}{120}\cdot A_4(5,1)-\frac{2}{120}\cdot A_4(5,4)-\frac{2}{120}\cdot A_4(6,1)-\frac{2}{120}\cdot A_4(6,3)-\frac{2}{120}\cdot A_4(7,1)-\frac{2}{120}\cdot A_4(7,2)$$

$$=\frac{8}{120\cdot 4(1/3)^3}+\frac{0}{120\cdot 5(2/3)^4}-\frac{2}{120}\cdot\frac{83816640}{53084160}-\frac{2}{120}\cdot\frac{83816640}{53084160}-\frac{2}{120}\cdot\frac{233625600}{53084160}-\frac{2}{120}\cdot\frac{83816640}{53084160}$$
$$-\frac{2}{120}\cdot\frac{359826702}{53084160}-\frac{2}{120}\cdot\frac{83816640}{53084160}-\frac{2}{120}\cdot\frac{359826702}{53084160}-\frac{2}{120}\cdot\frac{233625600}{53084160}+\frac{2}{120}\cdot\frac{3815424}{53084160}+\frac{2}{120}\cdot\frac{4455024}{53084160}$$
$$+\frac{2}{120}\cdot\frac{3815424}{53084160}+\frac{2}{120}\cdot\frac{4455024}{53084160}+\frac{2}{120}\cdot\frac{3815424}{53084160}+\frac{2}{120}\cdot\frac{3815424}{53084160}+\frac{2}{120}\cdot\frac{4455024}{53084160}+\frac{2}{120}\cdot\frac{4455024}{53084160}$$
$$+\frac{2}{120}\cdot\frac{54645562}{53084160}+\frac{2}{120}\cdot\frac{54645562}{53084160}+\frac{2}{120}\cdot\frac{54645562}{53084160}+\frac{2}{120}\cdot\frac{69672960}{53084160}+\frac{2}{120}\cdot\frac{69672960}{53084160}+\frac{2}{120}\cdot\frac{69672960}{53084160}$$
$$+\frac{2}{120}\cdot\frac{54645562}{53084160}+\frac{2}{120}\cdot\frac{69672960}{53084160}+\frac{2}{120}\cdot\frac{54645562}{53084160}+\frac{2}{120}\cdot\frac{69672960}{53084160}+\frac{2}{120}\cdot\frac{54645562}{53084160}+\frac{2}{120}\cdot\frac{69672960}{53084160}$$

$$=\frac{13}{60}.$$

$J_{23}$ : 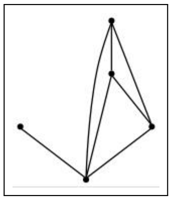

$$\frac{t_{\mathrm{inj}}(C_4, J_{23})}{4(1/3)^3} + \frac{t_{\mathrm{inj}}(C_5, \overline{J_{23}})}{5(2/3)^4} - \frac{6}{120}\cdot A_2(5,8) - \frac{6}{120}\cdot A_2(8,5) - \frac{6}{120}\cdot A_3(5,5) - \frac{6}{120}\cdot A_3(6,6)$$
$$-\frac{6}{120}\cdot A_4(1,8) - \frac{6}{120}\cdot A_4(2,8) - \frac{6}{120}\cdot A_4(3,8) - \frac{6}{120}\cdot A_4(4,8) - \frac{6}{120}\cdot A_4(8,1) - \frac{6}{120}\cdot A_4(8,2)$$
$$-\frac{6}{120}\cdot A_4(8,3) - \frac{6}{120}\cdot A_4(8,4)$$
$$= \frac{24}{120\cdot 4(1/3)^3} + \frac{0}{120\cdot 5(2/3)^4} - \frac{6}{120}\cdot\frac{233625600}{53084160} - \frac{6}{120}\cdot\frac{233625600}{53084160} - \frac{6}{120}\cdot\frac{466255872}{53084160} - \frac{6}{120}\cdot\frac{466255872}{53084160}$$
$$+\frac{6}{120}\cdot\frac{93533184}{53084160} + \frac{6}{120}\cdot\frac{1575936}{53084160} + \frac{6}{120}\cdot\frac{1575936}{53084160} + \frac{6}{120}\cdot\frac{1575936}{53084160} + \frac{6}{120}\cdot\frac{93533184}{53084160} + \frac{6}{120}\cdot\frac{1575936}{53084160}$$
$$+\frac{6}{120}\cdot\frac{1575936}{53084160} + \frac{6}{120}\cdot\frac{1575936}{53084160}$$
$$= \frac{13}{60}.$$

$J_{24}$ : 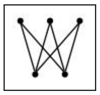

$$\frac{t_{\mathrm{inj}}(C_4, J_{24})}{4(1/3)^3} + \frac{t_{\mathrm{inj}}(C_5, \overline{J_{24}})}{5(2/3)^4} - \frac{12}{120}\cdot A_1(8,8) - \frac{12}{120}\cdot A_3(2,7) - \frac{12}{120}\cdot A_3(7,2) - \frac{12}{120}\cdot A_3(7,7)$$
$$= \frac{24}{120\cdot 4(1/3)^3} + \frac{0}{120\cdot 5(2/3)^4} - \frac{12}{120}\cdot\frac{312532992}{53084160} + \frac{12}{120}\cdot\frac{39429504}{53084160} + \frac{12}{120}\cdot\frac{39429504}{53084160} - \frac{12}{120}\cdot\frac{367946496}{53084160}$$
$$= \frac{13}{60}.$$

$J_{25}$ : 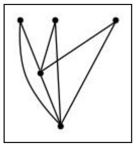

$$\frac{t_{\mathrm{inj}}(C_4, J_{25})}{4(1/3)^3} + \frac{t_{\mathrm{inj}}(C_5, \overline{J_{25}})}{5(2/3)^4} - \frac{12}{120}\cdot A_1(8,8) - \frac{12}{120}\cdot A_3(2,8) - \frac{12}{120}\cdot A_3(8,2) - \frac{12}{120}\cdot A_4(5,5)$$

$$-\frac{12}{120}\cdot A_4(6,6)-\frac{12}{120}\cdot A_4(7,7)$$

$$=\frac{24}{120\cdot 4(1/3)^3}+\frac{0}{120\cdot 5(2/3)^4}-\frac{12}{120}\cdot\frac{312532992}{53084160}+\frac{12}{120}\cdot\frac{177831936}{53084160}+\frac{12}{120}\cdot\frac{177831936}{53084160}-\frac{12}{120}\cdot\frac{214917120}{53084160}$$

$$-\frac{12}{120}\cdot\frac{214917120}{53084160}-\frac{12}{120}\cdot\frac{214917120}{53084160}$$

$$=\frac{13}{60}.$$

$J_{26}$ : 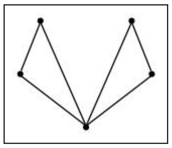

$$\frac{t_{\text{inj}}(C_4,J_{26})}{4(1/3)^3}+\frac{t_{\text{inj}}(C_5,\overline{J_{26}})}{5(2/3)^4}-\frac{8}{120}\cdot A_2(4,8)-\frac{8}{120}\cdot A_2(8,4)-\frac{8}{120}\cdot A_3(5,6)-\frac{8}{120}\cdot A_3(6,5)$$

$$-\frac{8}{120}\cdot A_4(2,2)-\frac{8}{120}\cdot A_4(3,3)-\frac{8}{120}\cdot A_4(4,4)$$

$$=\frac{0}{120\cdot 4(1/3)^3}+\frac{0}{120\cdot 5(2/3)^4}+\frac{8}{120}\cdot\frac{198826518}{53084160}+\frac{8}{120}\cdot\frac{198826518}{53084160}+\frac{8}{120}\cdot\frac{44568576}{53084160}+\frac{8}{120}\cdot\frac{44568576}{53084160}$$

$$-\frac{8}{120}\cdot\frac{104755556}{53084160}-\frac{8}{120}\cdot\frac{104755556}{53084160}-\frac{8}{120}\cdot\frac{104755556}{53084160}$$

$$=\frac{13}{60}.$$

$J_{27}$ : 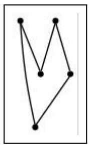

$$\frac{t_{\text{inj}}(C_4,J_{27})}{4(1/3)^3}+\frac{t_{\text{inj}}(C_5,\overline{J_{27}})}{5(2/3)^4}-\frac{10}{120}\cdot A_2(6,7)-\frac{10}{120}\cdot A_2(7,6)-\frac{10}{120}\cdot A_3(3,4)-\frac{10}{120}\cdot A_3(4,3)$$

$$=\frac{0}{120\cdot 4(1/3)^3}+\frac{10}{120\cdot 5(2/3)^4}-\frac{10}{120}\cdot\frac{20736000}{53084160}-\frac{10}{120}\cdot\frac{20736000}{53084160}+\frac{10}{120}\cdot\frac{62871552}{53084160}+\frac{10}{120}\cdot\frac{62871552}{53084160}$$

$$=\frac{13}{60}.$$

$J_{28}$ : 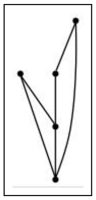

$$\frac{t_{\text{inj}}(C_4, J_{28})}{4(1/3)^3} + \frac{t_{\text{inj}}(C_5, \overline{J_{28}})}{5(2/3)^4} - \frac{2}{120} \cdot A_2(6,7) - \frac{2}{120} \cdot A_2(6,8) - \frac{2}{120} \cdot A_2(7,6) - \frac{2}{120} \cdot A_2(7,8)$$

$$-\frac{2}{120} \cdot A_2(8,6) - \frac{2}{120} \cdot A_2(8,7) - \frac{2}{120} \cdot A_3(3,6) - \frac{2}{120} \cdot A_3(3,7) - \frac{2}{120} \cdot A_3(4,5) - \frac{2}{120} \cdot A_3(4,7)$$
$$-\frac{2}{120} \cdot A_3(5,4) - \frac{2}{120} \cdot A_3(5,7) - \frac{2}{120} \cdot A_3(6,3) - \frac{2}{120} \cdot A_3(6,7) - \frac{2}{120} \cdot A_3(7,3) - \frac{2}{120} \cdot A_3(7,4)$$
$$-\frac{2}{120} \cdot A_3(7,5) - \frac{2}{120} \cdot A_3(7,6) - \frac{2}{120} \cdot A_4(2,3) - \frac{2}{120} \cdot A_4(2,4) - \frac{2}{120} \cdot A_4(3,2) - \frac{2}{120} \cdot A_4(3,4)$$
$$-\frac{2}{120} \cdot A_4(4,2) - \frac{2}{120} \cdot A_4(4,3)$$
$$= \frac{8}{120 \cdot 4(1/3)^3} + \frac{0}{120 \cdot 5(2/3)^4} - \frac{2}{120} \cdot \frac{20736000}{53084160} - \frac{2}{120} \cdot \frac{244463616}{53084160} - \frac{2}{120} \cdot \frac{20736000}{53084160} - \frac{2}{120} \cdot \frac{244463616}{53084160}$$
$$-\frac{2}{120} \cdot \frac{244463616}{53084160} - \frac{2}{120} \cdot \frac{244463616}{53084160} + \frac{2}{120} \cdot \frac{96242688}{53084160} + \frac{2}{120} \cdot \frac{30360144}{53084160} + \frac{2}{120} \cdot \frac{96242688}{53084160} + \frac{2}{120} \cdot \frac{30360144}{53084160}$$
$$+\frac{2}{120} \cdot \frac{96242688}{53084160} - \frac{2}{120} \cdot \frac{109264896}{53084160} + \frac{2}{120} \cdot \frac{96242688}{53084160} - \frac{2}{120} \cdot \frac{109264896}{53084160} + \frac{2}{120} \cdot \frac{30360144}{53084160} + \frac{2}{120} \cdot \frac{30360144}{53084160}$$
$$-\frac{2}{120} \cdot \frac{109264896}{53084160} - \frac{2}{120} \cdot \frac{109264896}{53084160} + \frac{2}{120} \cdot \frac{34466080}{53084160} + \frac{2}{120} \cdot \frac{34466080}{53084160} + \frac{2}{120} \cdot \frac{34466080}{53084160} + \frac{2}{120} \cdot \frac{34466080}{53084160}$$
$$+\frac{2}{120} \cdot \frac{34466080}{53084160} + \frac{2}{120} \cdot \frac{34466080}{53084160}$$
$$= \frac{13}{60}.$$

$J_{29}$ : 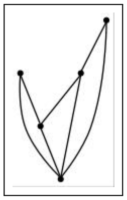

$$\frac{t_{\text{inj}}(C_4, J_{29})}{4(1/3)^3} + \frac{t_{\text{inj}}(C_5, \overline{J_{29}})}{5(2/3)^4} - \frac{2}{120} \cdot A_2(6,8) - \frac{2}{120} \cdot A_2(7,8) - \frac{2}{120} \cdot A_2(8,6) - \frac{2}{120} \cdot A_2(8,7)$$

$$-\frac{2}{120} \cdot A_3(3,8) - \frac{2}{120} \cdot A_3(4,8) - \frac{2}{120} \cdot A_3(5,6) - \frac{2}{120} \cdot A_3(5,8) - \frac{2}{120} \cdot A_3(6,5) - \frac{2}{120} \cdot A_3(6,8)$$

$$-\frac{2}{120}\cdot A_3(8,3)-\frac{2}{120}\cdot A_3(8,4)-\frac{2}{120}\cdot A_3(8,5)-\frac{2}{120}\cdot A_3(8,6)-\frac{2}{120}\cdot A_4(2,5)-\frac{2}{120}\cdot A_4(2,6)$$
$$-\frac{2}{120}\cdot A_4(3,5)-\frac{2}{120}\cdot A_4(3,7)-\frac{2}{120}\cdot A_4(4,6)-\frac{2}{120}\cdot A_4(4,7)-\frac{2}{120}\cdot A_4(5,2)-\frac{2}{120}\cdot A_4(5,3)$$
$$-\frac{2}{120}\cdot A_4(5,6)-\frac{2}{120}\cdot A_4(5,7)-\frac{2}{120}\cdot A_4(6,2)-\frac{2}{120}\cdot A_4(6,4)-\frac{2}{120}\cdot A_4(6,5)-\frac{2}{120}\cdot A_4(6,7)$$
$$-\frac{2}{120}\cdot A_4(7,3)-\frac{2}{120}\cdot A_4(7,4)-\frac{2}{120}\cdot A_4(7,5)-\frac{2}{120}\cdot A_4(7,6)$$
$$=\frac{16}{120\cdot 4(1/3)^3}+\frac{0}{120\cdot 5(2/3)^4}-\frac{2}{120}\cdot\frac{244463616}{53084160}-\frac{2}{120}\cdot\frac{244463616}{53084160}-\frac{2}{120}\cdot\frac{244463616}{53084160}-\frac{2}{120}\cdot\frac{244463616}{53084160}$$
$$+\frac{2}{120}\cdot\frac{4455024}{53084160}+\frac{2}{120}\cdot\frac{4455024}{53084160}+\frac{2}{120}\cdot\frac{44568576}{53084160}-\frac{2}{120}\cdot\frac{245402496}{53084160}+\frac{2}{120}\cdot\frac{44568576}{53084160}-\frac{2}{120}\cdot\frac{245402496}{53084160}$$
$$+\frac{2}{120}\cdot\frac{4455024}{53084160}+\frac{2}{120}\cdot\frac{4455024}{53084160}-\frac{2}{120}\cdot\frac{245402496}{53084160}-\frac{2}{120}\cdot\frac{245402496}{53084160}-\frac{2}{120}\cdot\frac{15801488}{53084160}-\frac{2}{120}\cdot\frac{15801488}{53084160}$$
$$-\frac{2}{120}\cdot\frac{15801488}{53084160}-\frac{2}{120}\cdot\frac{15801488}{53084160}-\frac{2}{120}\cdot\frac{15801488}{53084160}-\frac{2}{120}\cdot\frac{15801488}{53084160}-\frac{2}{120}\cdot\frac{15801488}{53084160}-\frac{2}{120}\cdot\frac{15801488}{53084160}$$
$$-\frac{2}{120}\cdot\frac{22387584}{53084160}-\frac{2}{120}\cdot\frac{22387584}{53084160}-\frac{2}{120}\cdot\frac{15801488}{53084160}-\frac{2}{120}\cdot\frac{15801488}{53084160}-\frac{2}{120}\cdot\frac{22387584}{53084160}-\frac{2}{120}\cdot\frac{22387584}{53084160}$$
$$-\frac{2}{120}\cdot\frac{15801488}{53084160}-\frac{2}{120}\cdot\frac{15801488}{53084160}-\frac{2}{120}\cdot\frac{22387584}{53084160}-\frac{2}{120}\cdot\frac{22387584}{53084160}$$
$$=\frac{13}{60}.$$

$J_{30}$ : 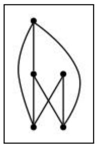

$$\frac{t_{\mathrm{inj}}(C_4,J_{30})}{4(1/3)^3}+\frac{t_{\mathrm{inj}}(C_5,\overline{J_{30}})}{5(2/3)^4}-\frac{4}{120}\cdot A_2(8,8)-\frac{4}{120}\cdot A_3(5,7)-\frac{4}{120}\cdot A_3(6,7)-\frac{4}{120}\cdot A_3(7,5)$$
$$-\frac{4}{120}\cdot A_3(7,6)-\frac{4}{120}\cdot A_3(7,7)-\frac{4}{120}\cdot A_3(7,8)-\frac{4}{120}\cdot A_3(8,7)-\frac{4}{120}\cdot A_4(2,7)-\frac{4}{120}\cdot A_4(3,6)$$
$$-\frac{4}{120}\cdot A_4(4,5)-\frac{4}{120}\cdot A_4(5,4)-\frac{4}{120}\cdot A_4(6,3)-\frac{4}{120}\cdot A_4(7,2)$$
$$=\frac{24}{120\cdot 4(1/3)^3}+\frac{0}{120\cdot 5(2/3)^4}-\frac{4}{120}\cdot\frac{1200867840}{53084160}-\frac{4}{120}\cdot\frac{109264896}{53084160}-\frac{4}{120}\cdot\frac{109264896}{53084160}-\frac{4}{120}\cdot\frac{109264896}{53084160}$$
$$-\frac{4}{120}\cdot\frac{109264896}{53084160}-\frac{4}{120}\cdot\frac{367946496}{53084160}-\frac{4}{120}\cdot\frac{108512640}{53084160}-\frac{4}{120}\cdot\frac{108512640}{53084160}+\frac{4}{120}\cdot\frac{69672960}{53084160}+\frac{4}{120}\cdot\frac{69672960}{53084160}$$
$$+\frac{4}{120}\cdot\frac{69672960}{53084160}+\frac{4}{120}\cdot\frac{69672960}{53084160}+\frac{4}{120}\cdot\frac{69672960}{53084160}+\frac{4}{120}\cdot\frac{69672960}{53084160}$$

$$= \frac{13}{60}.$$

$J_{31}$ : 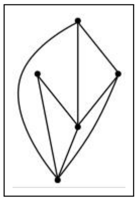

$$\frac{t_{\text{inj}}(C_4, J_{31})}{4(1/3)^3} + \frac{t_{\text{inj}}(C_5, \overline{J_{31}})}{5(2/3)^4} - \frac{4}{120} \cdot A_2(8,8) - \frac{4}{120} \cdot A_3(5,8) - \frac{4}{120} \cdot A_3(6,8) - \frac{4}{120} \cdot A_3(8,5)$$
$$- \frac{4}{120} \cdot A_3(8,6) - \frac{4}{120} \cdot A_4(2,8) - \frac{4}{120} \cdot A_4(3,8) - \frac{4}{120} \cdot A_4(4,8) - \frac{4}{120} \cdot A_4(5,5) - \frac{4}{120} \cdot A_4(5,8)$$
$$- \frac{4}{120} \cdot A_4(6,6) - \frac{4}{120} \cdot A_4(6,8) - \frac{4}{120} \cdot A_4(7,7) - \frac{4}{120} \cdot A_4(7,8) - \frac{4}{120} \cdot A_4(8,2) - \frac{4}{120} \cdot A_4(8,3)$$
$$- \frac{4}{120} \cdot A_4(8,4) - \frac{4}{120} \cdot A_4(8,5) - \frac{4}{120} \cdot A_4(8,6) - \frac{4}{120} \cdot A_4(8,7)$$
$$= \frac{40}{120 \cdot 4(1/3)^3} + \frac{0}{120 \cdot 5(2/3)^4} - \frac{4}{120} \cdot \frac{1200867840}{53084160} - \frac{4}{120} \cdot \frac{245402496}{53084160} - \frac{4}{120} \cdot \frac{245402496}{53084160} - \frac{4}{120} \cdot \frac{245402496}{53084160}$$
$$- \frac{4}{120} \cdot \frac{245402496}{53084160} + \frac{4}{120} \cdot \frac{1575936}{53084160} + \frac{4}{120} \cdot \frac{1575936}{53084160} + \frac{4}{120} \cdot \frac{1575936}{53084160} - \frac{4}{120} \cdot \frac{214917120}{53084160} - \frac{4}{120} \cdot \frac{70060032}{53084160}$$
$$- \frac{4}{120} \cdot \frac{214917120}{53084160} - \frac{4}{120} \cdot \frac{70060032}{53084160} - \frac{4}{120} \cdot \frac{214917120}{53084160} - \frac{4}{120} \cdot \frac{70060032}{53084160} + \frac{4}{120} \cdot \frac{1575936}{53084160} + \frac{4}{120} \cdot \frac{1575936}{53084160}$$
$$+ \frac{4}{120} \cdot \frac{1575936}{53084160} - \frac{4}{120} \cdot \frac{70060032}{53084160} - \frac{4}{120} \cdot \frac{70060032}{53084160} - \frac{4}{120} \cdot \frac{70060032}{53084160}$$
$$= \frac{13}{60}.$$

$J_{32}$ : 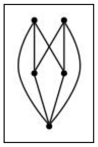

$$\frac{t_{\text{inj}}(C_4, J_{32})}{4(1/3)^3} + \frac{t_{\text{inj}}(C_5, \overline{J_{32}})}{5(2/3)^4} - \frac{8}{120} \cdot A_3(7,8) - \frac{8}{120} \cdot A_3(8,7) - \frac{8}{120} \cdot A_3(8,8) - \frac{8}{120} \cdot A_4(5,6)$$
$$- \frac{8}{120} \cdot A_4(5,7) - \frac{8}{120} \cdot A_4(6,5) - \frac{8}{120} \cdot A_4(6,7) - \frac{8}{120} \cdot A_4(7,5) - \frac{8}{120} \cdot A_4(7,6)$$
$$= \frac{40}{120 \cdot 4(1/3)^3} + \frac{0}{120 \cdot 5(2/3)^4} - \frac{8}{120} \cdot \frac{108512640}{53084160} - \frac{8}{120} \cdot \frac{108512640}{53084160} - \frac{8}{120} \cdot \frac{1267716096}{53084160} - \frac{8}{120} \cdot \frac{22387584}{53084160}$$
$$- \frac{8}{120} \cdot \frac{22387584}{53084160} - \frac{8}{120} \cdot \frac{22387584}{53084160} - \frac{8}{120} \cdot \frac{22387584}{53084160} - \frac{8}{120} \cdot \frac{22387584}{53084160} - \frac{8}{120} \cdot \frac{22387584}{53084160}$$

$$= \frac{13}{60}.$$

$J_{33}$ : 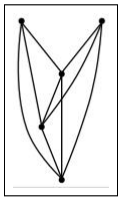

$$\frac{t_{\text{inj}}(C_4, J_{33})}{4(1/3)^3} + \frac{t_{\text{inj}}(C_5, \overline{J_{33}})}{5(2/3)^4} - \frac{12}{120} \cdot A_3(8,8) - \frac{12}{120} \cdot A_4(5,8) - \frac{12}{120} \cdot A_4(6,8) - \frac{12}{120} \cdot A_4(7,8)$$

$$- \frac{12}{120} \cdot A_4(8,5) - \frac{12}{120} \cdot A_4(8,6) - \frac{12}{120} \cdot A_4(8,7) - \frac{12}{120} \cdot A_4(8,8)$$

$$= \frac{72}{120 \cdot 4(1/3)^3} + \frac{0}{120 \cdot 5(2/3)^4} - \frac{12}{120} \cdot \frac{1267716096}{53084160} - \frac{12}{120} \cdot \frac{70060032}{53084160} - \frac{12}{120} \cdot \frac{70060032}{53084160} - \frac{12}{120} \cdot \frac{70060032}{53084160}$$

$$- \frac{12}{120} \cdot \frac{70060032}{53084160} - \frac{12}{120} \cdot \frac{70060032}{53084160} - \frac{12}{120} \cdot \frac{70060032}{53084160} - \frac{12}{120} \cdot \frac{346816512}{53084160}$$

$$= \frac{13}{60}.$$

$J_{34}$ : 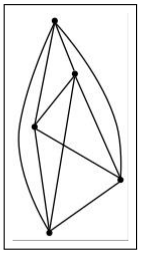

$$\frac{t_{\text{inj}}(C_4, J_{34})}{4(1/3)^3} + \frac{t_{\text{inj}}(C_5, \overline{J_{34}})}{5(2/3)^4} - \frac{120}{120} \cdot A_4(8,8)$$

$$= \frac{120}{120 \cdot 4(1/3)^3} + \frac{0}{120 \cdot 5(2/3)^4} - \frac{120}{120} \cdot \frac{346816512}{53084160}$$

$$= \frac{13}{60}.$$
